# Supplementary material for: Multimodal Knowledge Expansion
Source: arXiv:2103.14431 source file (2021-10-29)
Supplement: Supplementary file 1 [file supp2-exp.tex]

\section{Experimental Results}
\subsection{Emotion Recognition}
One interesting finding is presented in Figure \ref{fig:emo}. We compare the confusion matrix that the UM teacher, NOISY student and our MM student generates on test data. Compared with NOISY student, the MM student contributes quite differently for 8 classes: it significantly improves the class ``surprised'' and slightly improves over the ``neutral'' class. We hypothesize that audios belonging to class ``surprised'' have more distinct features than ``neutral'', and a multi-modal student effectively utilizes this information.

\subsection{Semantic Segmentation}
Figure \ref{fig:seg} presents more segmentation results on NYU Depth V2 test data. We can see that the UM Teacher generates inconsistent and noisy predictions, for instance, they fail to identify sofas in the third, fourth and sixth example. NOISY Student improves a little over the teacher's prediction. However, its prediction is still messy. In contrast, MM student identifies the sofa as a whole and gives mostly correct predictions. Depth modality here enables knowledge expansion from the RGB teacher.

\subsection{Event Classification}
\begin{table}[h]\small
	\centering
	\begin{tabular}{cccc}
		\toprule		
		& \multicolumn{3}{c}{Test mAP} \\
		&\makecell[c]{UM \\teacher}& \makecell[c]{NOISY \\student}&\makecell[c]{MM\\ student (ours)}\\
		\midrule
        % \rowcolor{mygray}
		basketball bounce&0.178& 0.263&0.542 \\
	    dog growling&0.069 & 0.096&0.516 \\
	   % \rowcolor{mygray}
	    people belly laughing& 0.334& 0.475 &0.800 \\
	    sliding door&0.104&0.163&0.388\\
	   % \rowcolor{mygray}
	    lawn mowing&0.318 &0.481 &0.541\\
		\bottomrule
	\end{tabular}
	\caption{Performance of top 5 event categories that MM student improves. Test mAP of the UM teacher and NOISY student are shown for comparison.}
	\label{tab:eventimprove}
\end{table}

\begin{figure*}[!htp]
\centering
\subfloat[RGB images]{
\begin{minipage}[b]{0.15\textwidth}
\centering
\includegraphics[scale=0.2]{./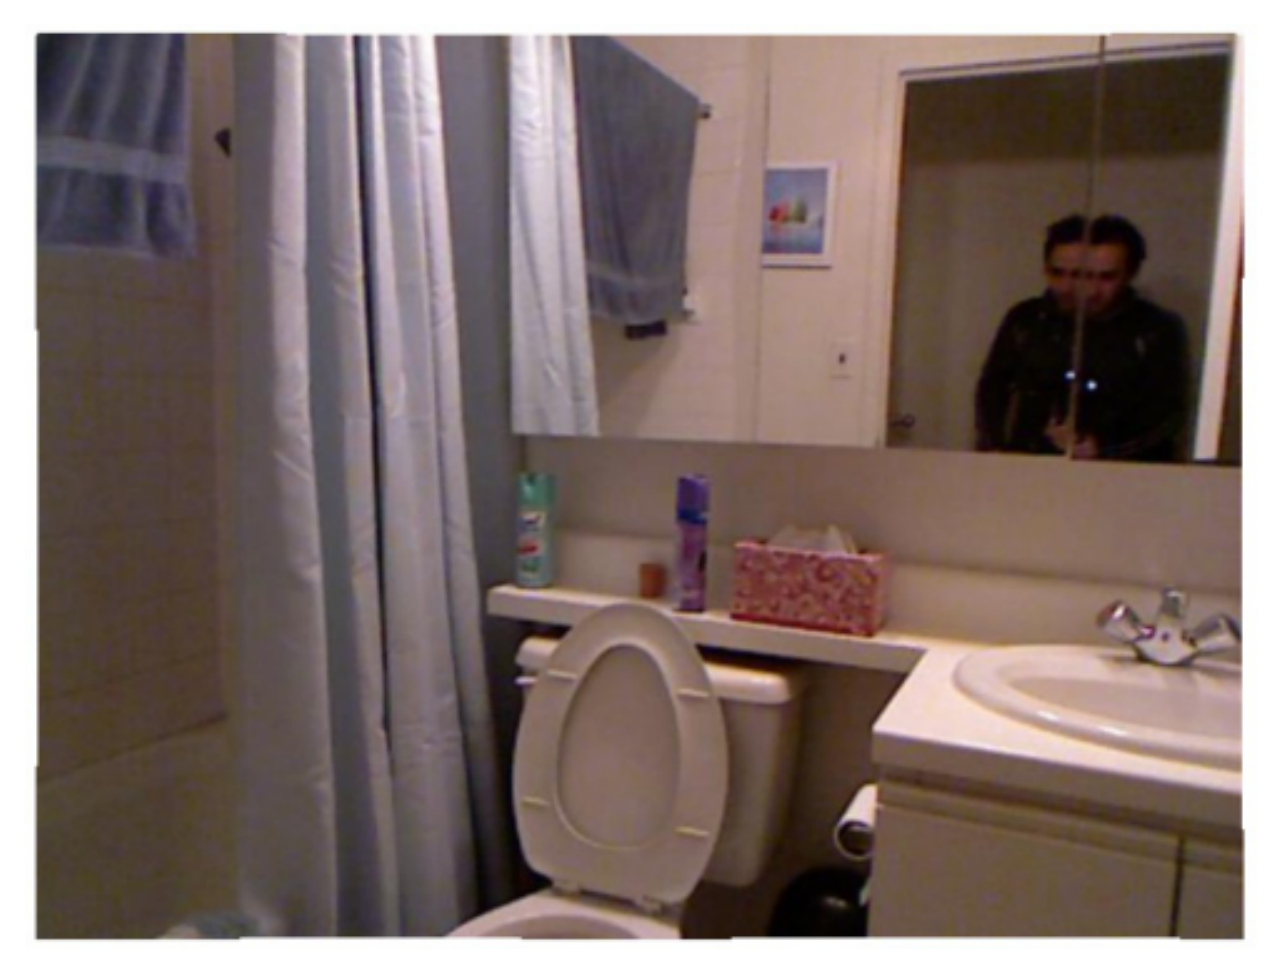} \\
\includegraphics[scale=0.2]{./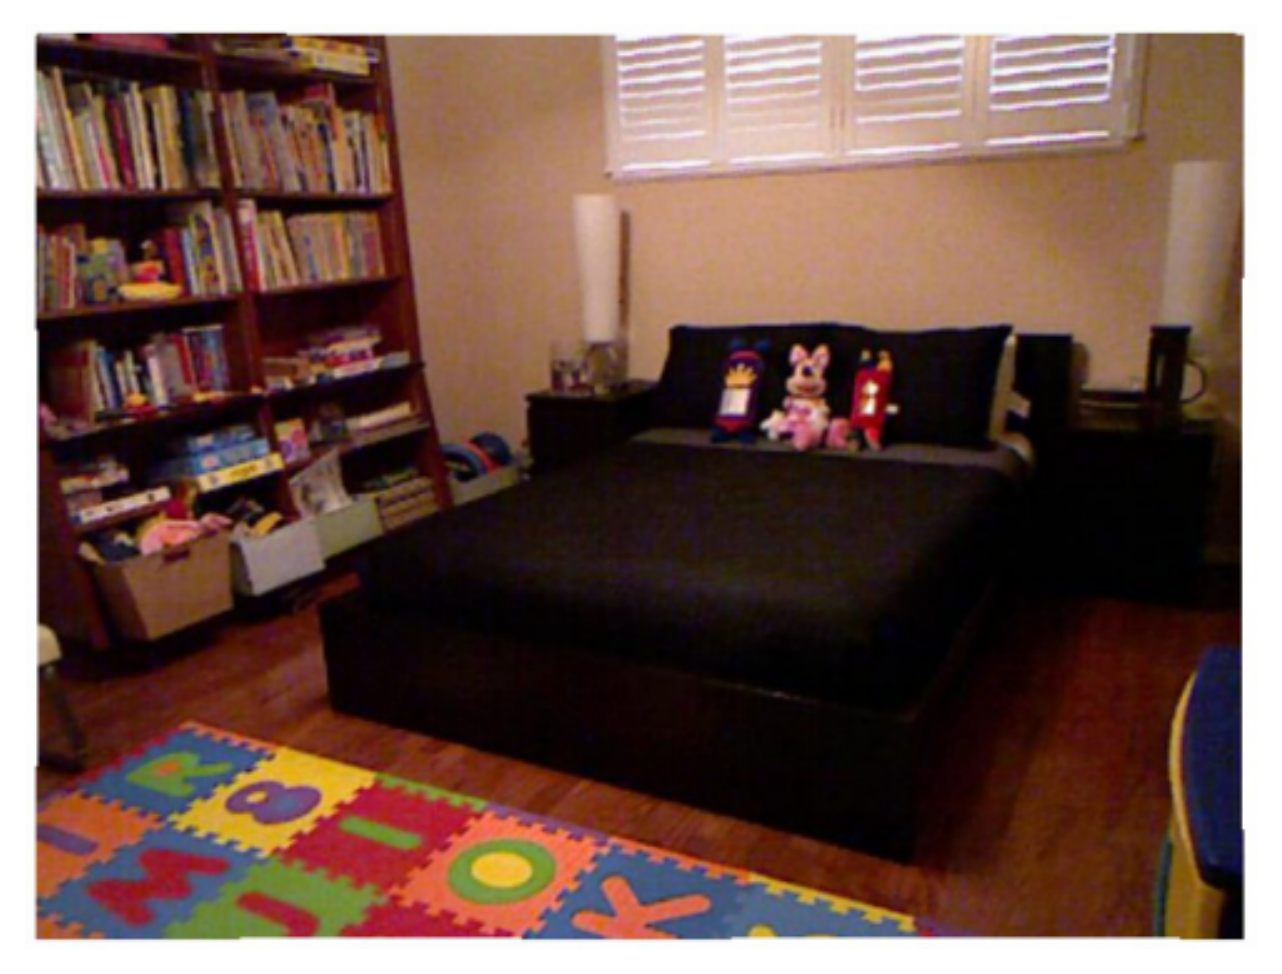} \\
\includegraphics[scale=0.2]{./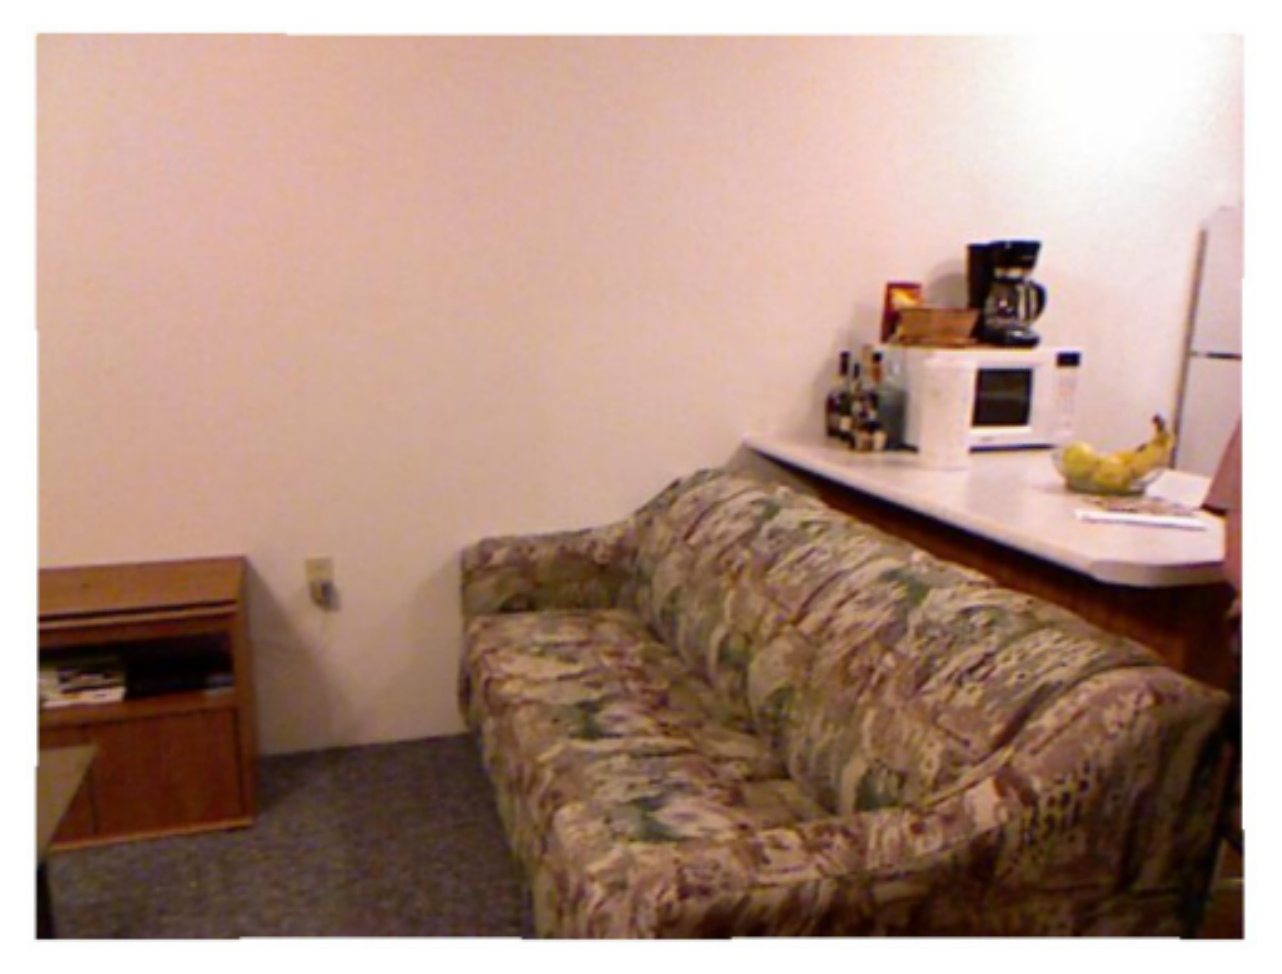} \\
\includegraphics[scale=0.2]{./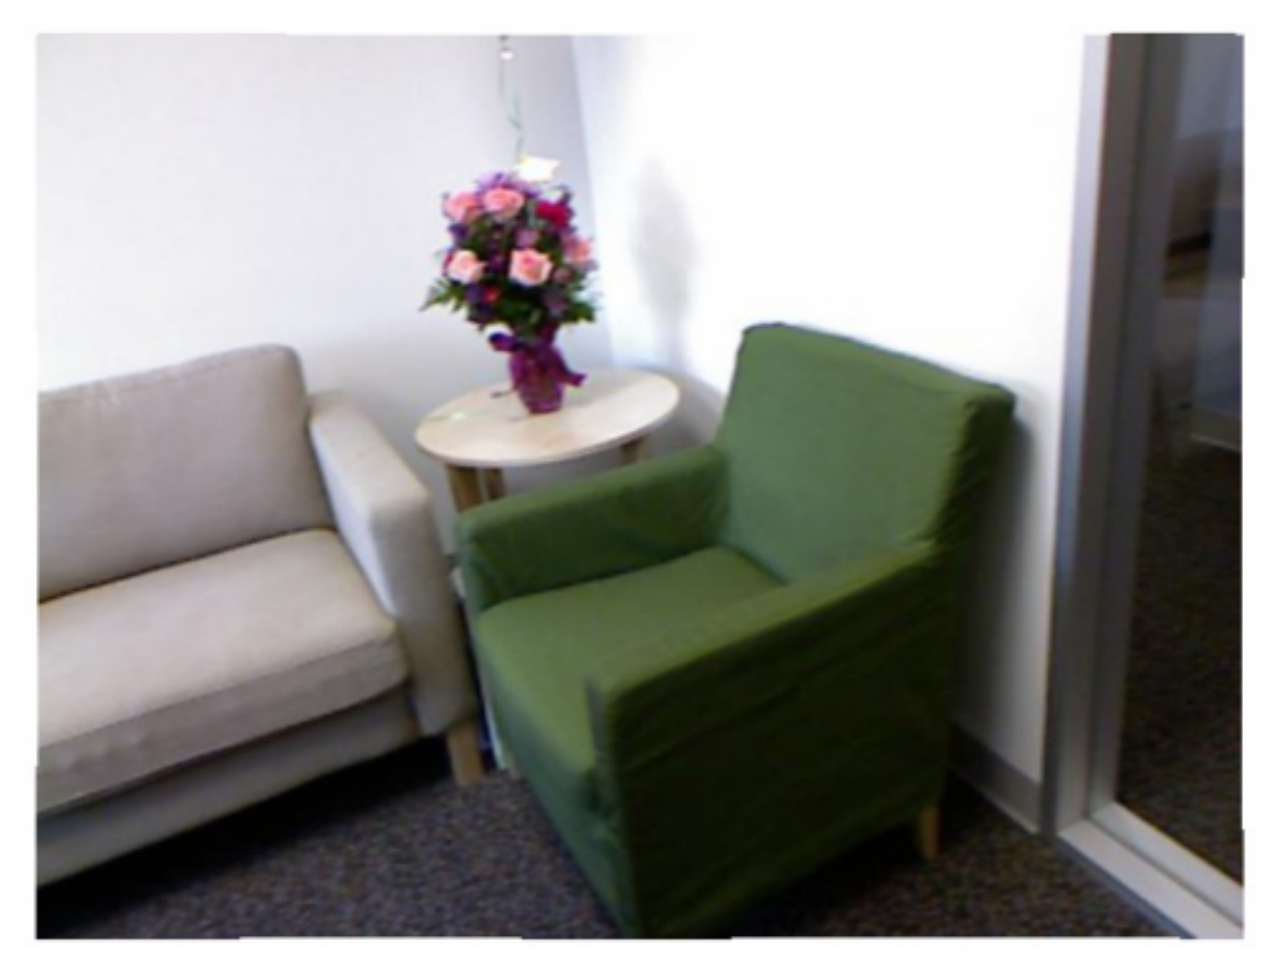} \\
\includegraphics[scale=0.2]{./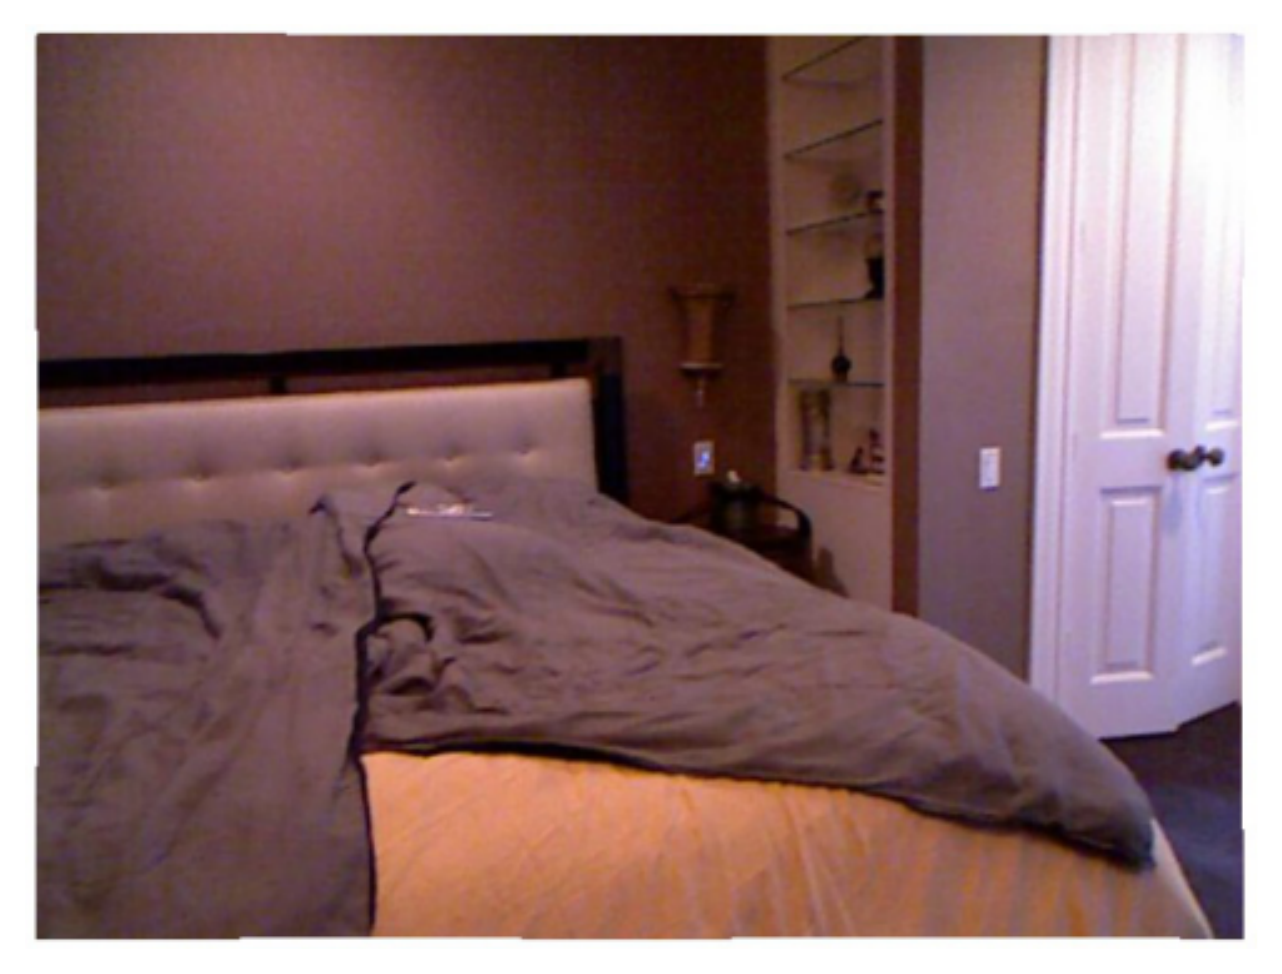} \\
\includegraphics[scale=0.2]{./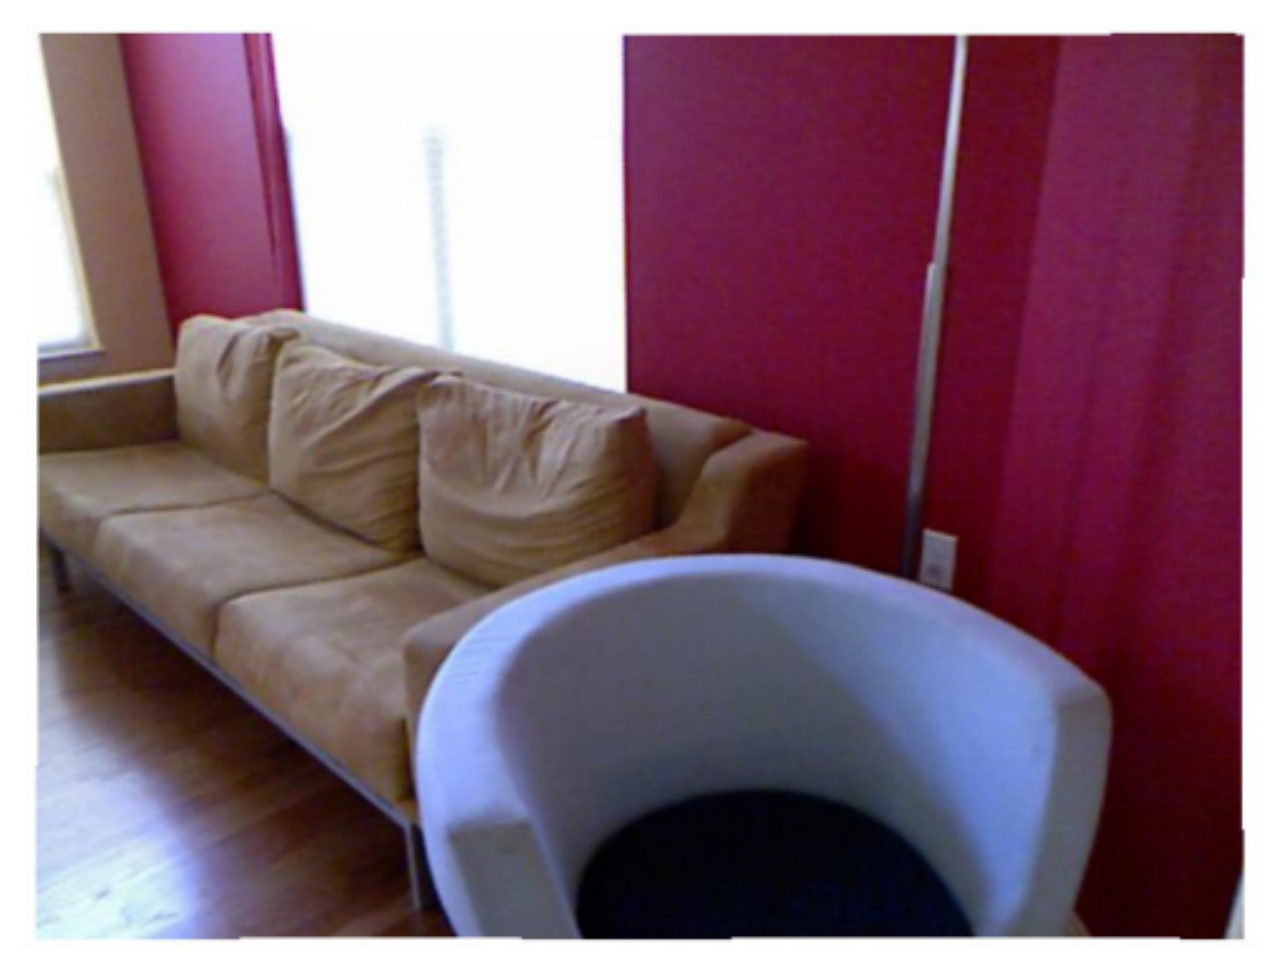} \\
\end{minipage}
}\hspace{-1.5mm}
\subfloat[depth images]{
\begin{minipage}[b]{0.15\textwidth}
\centering
\includegraphics[scale=0.2]{./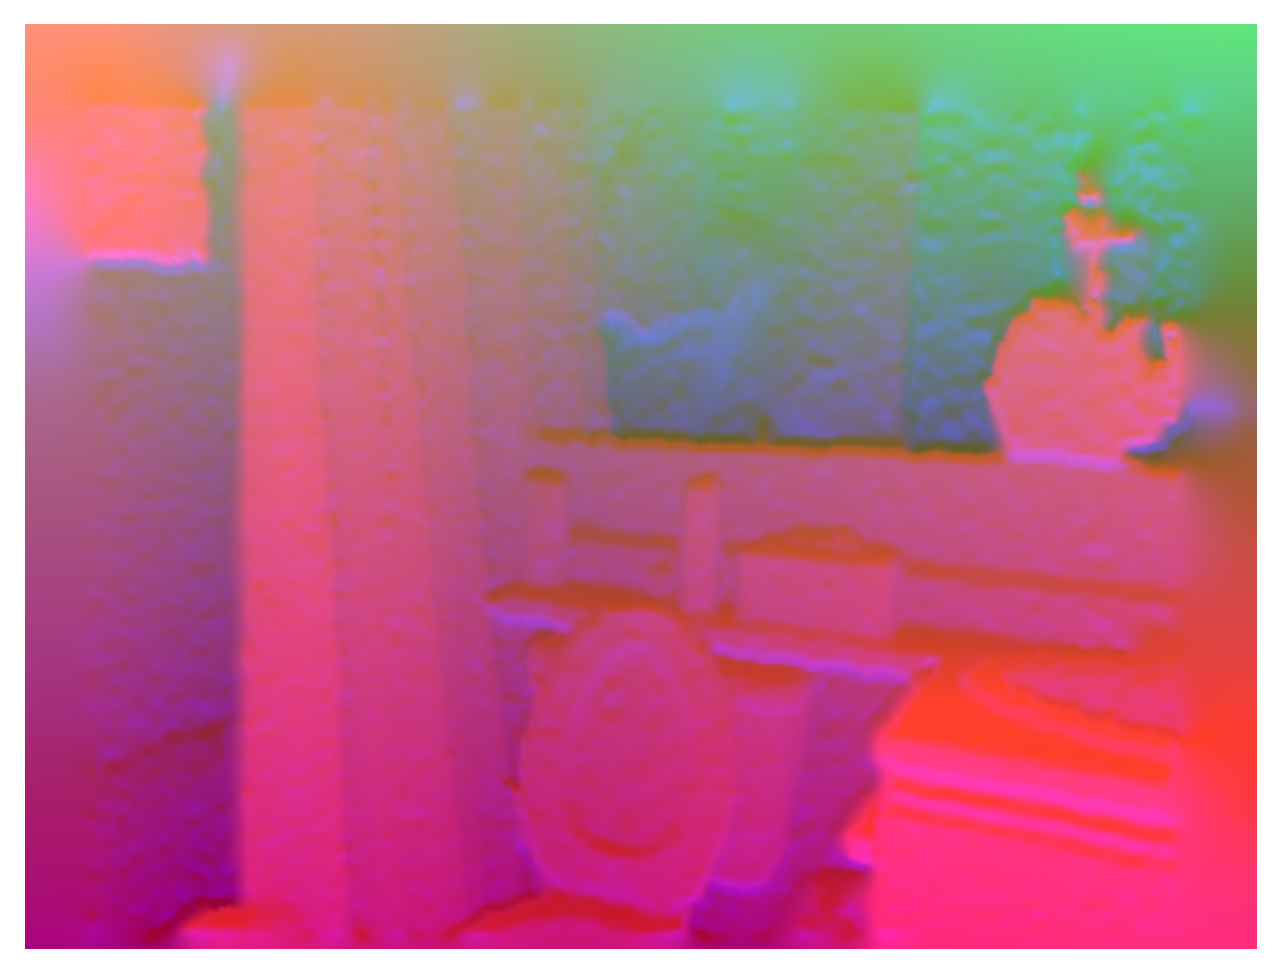} \\
\includegraphics[scale=0.2]{./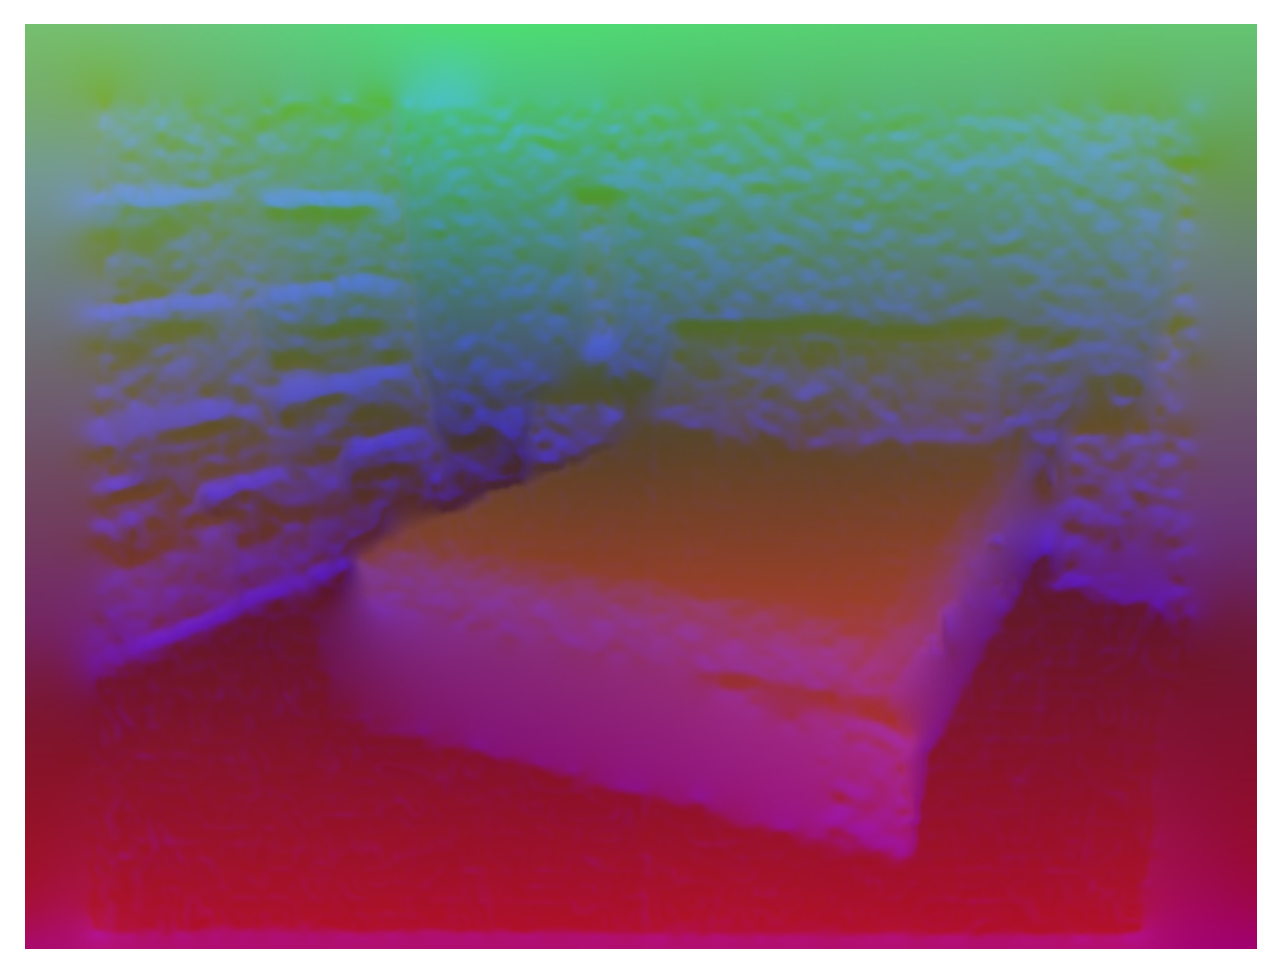} \\
\includegraphics[scale=0.2]{./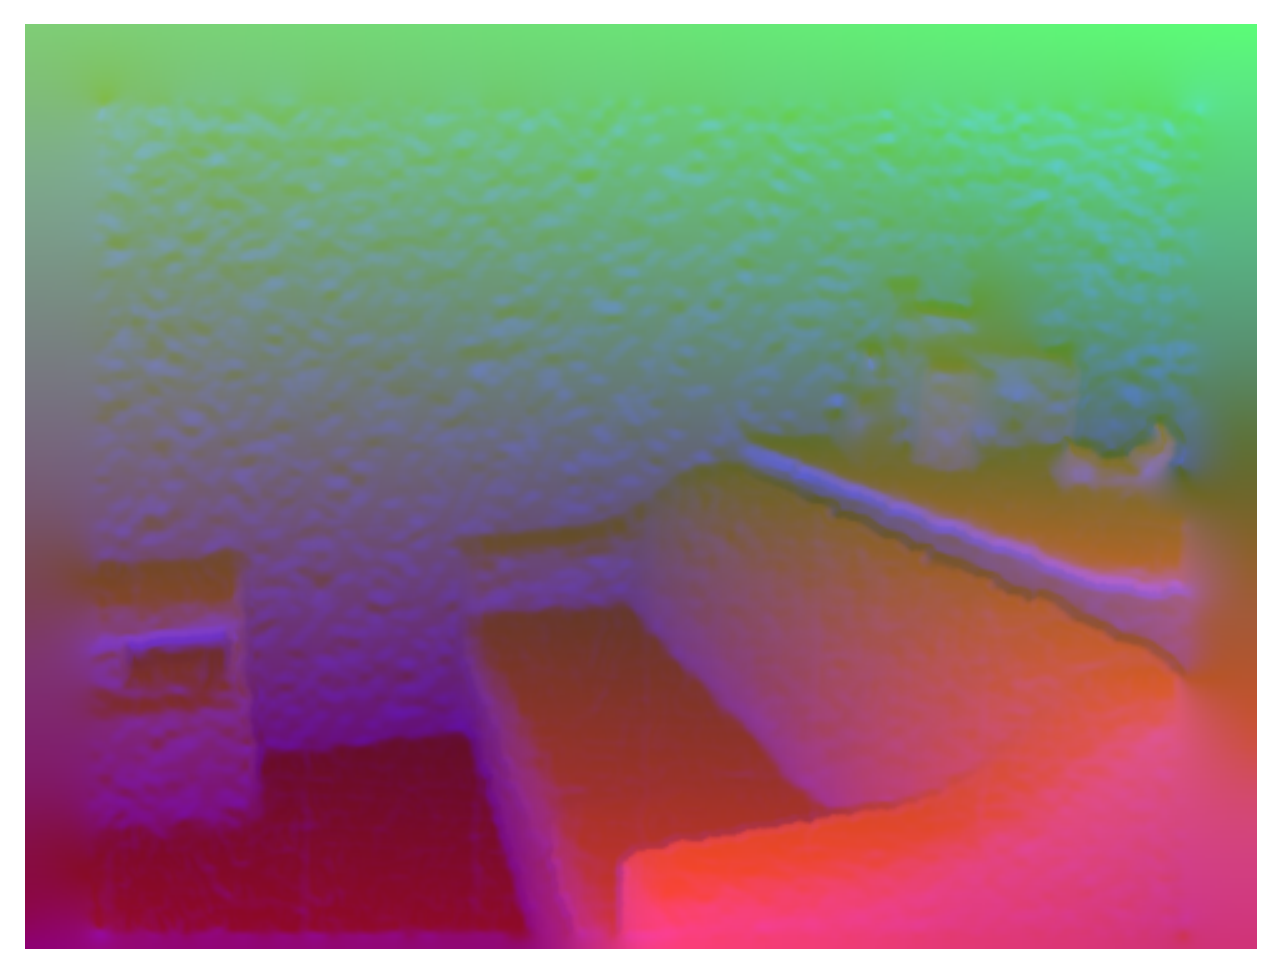} \\
\includegraphics[scale=0.2]{./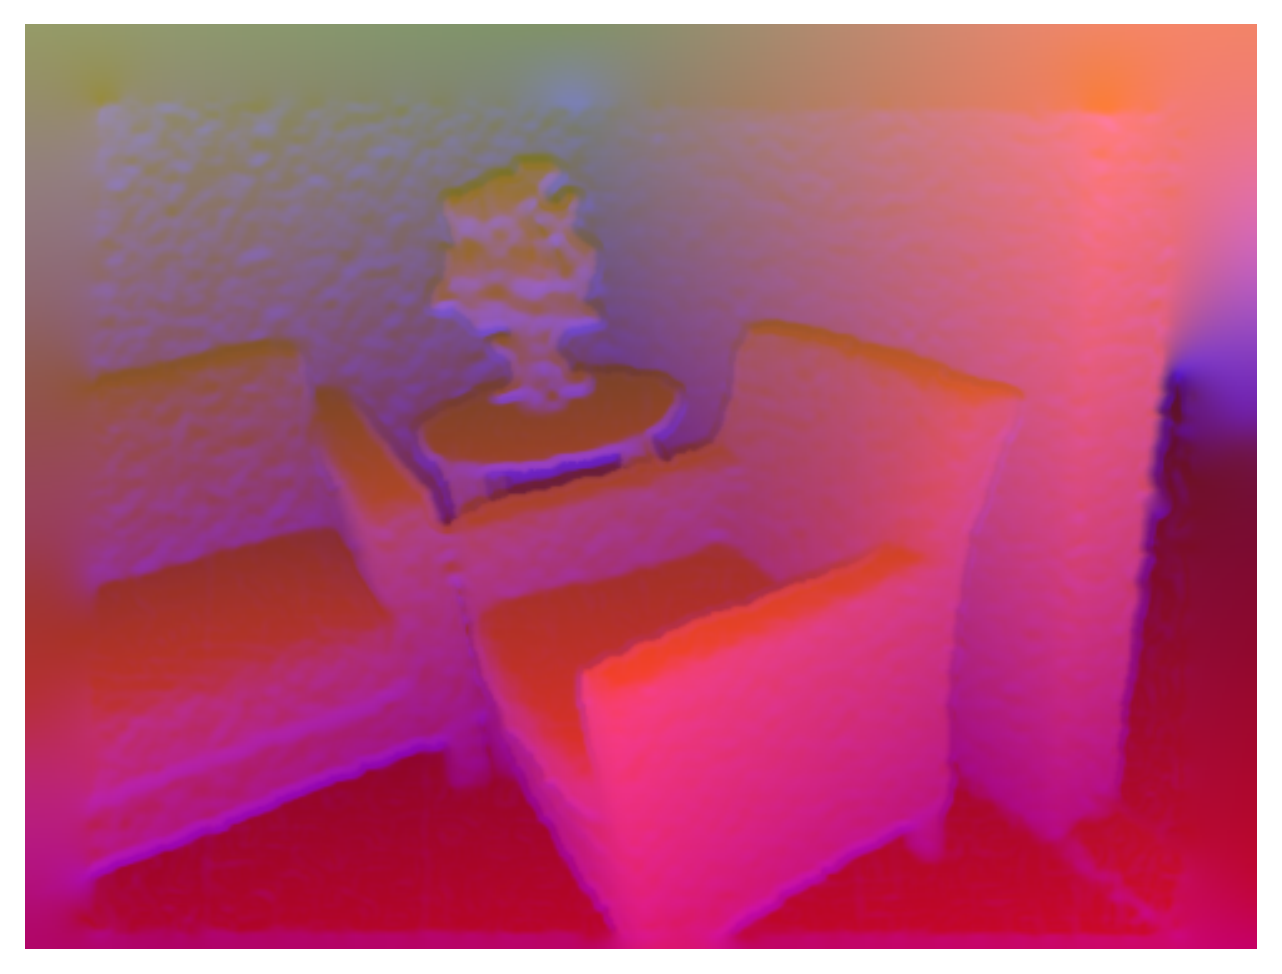} \\
\includegraphics[scale=0.2]{./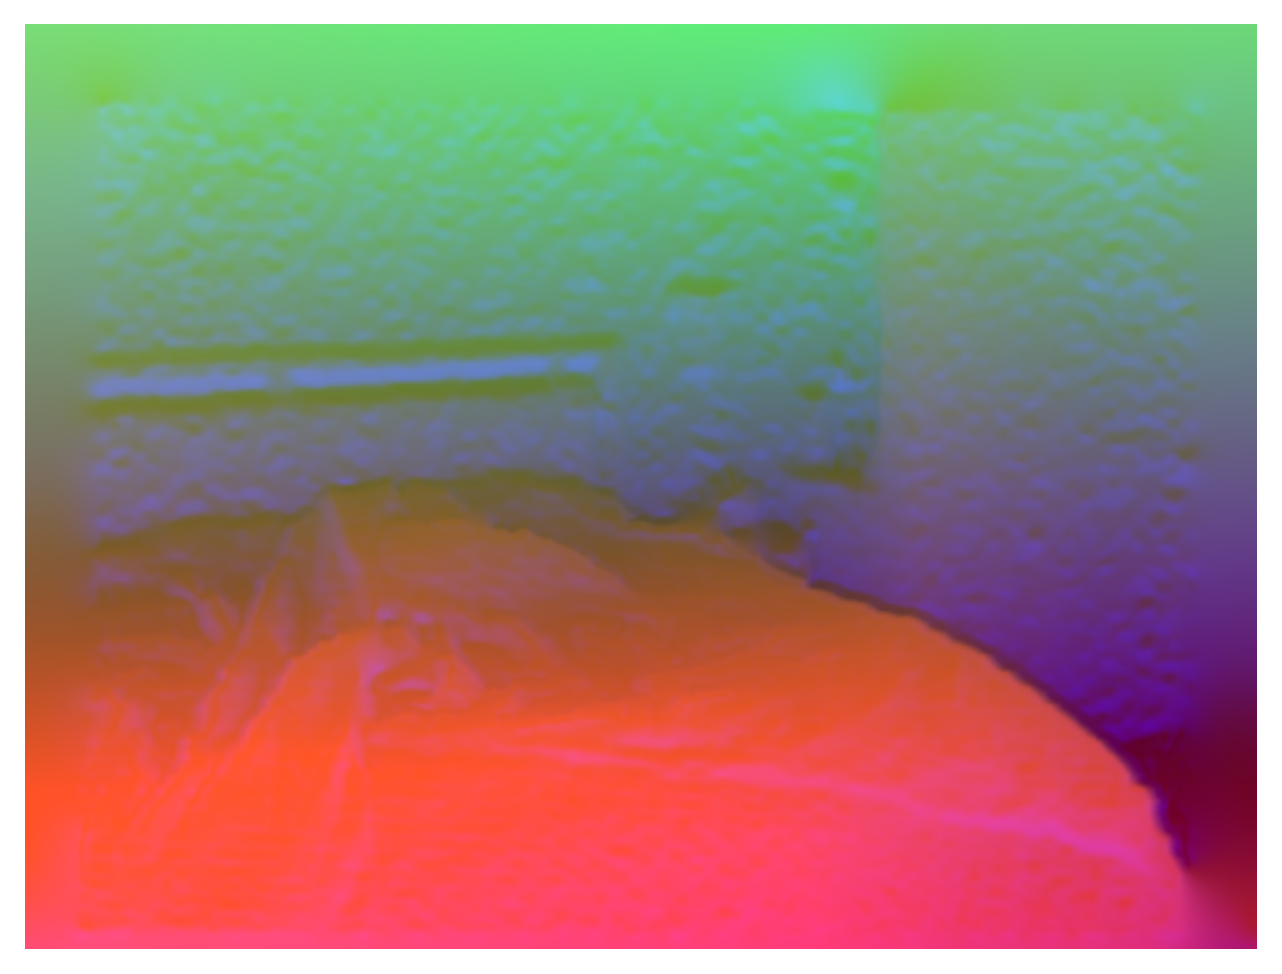} \\
\includegraphics[scale=0.2]{./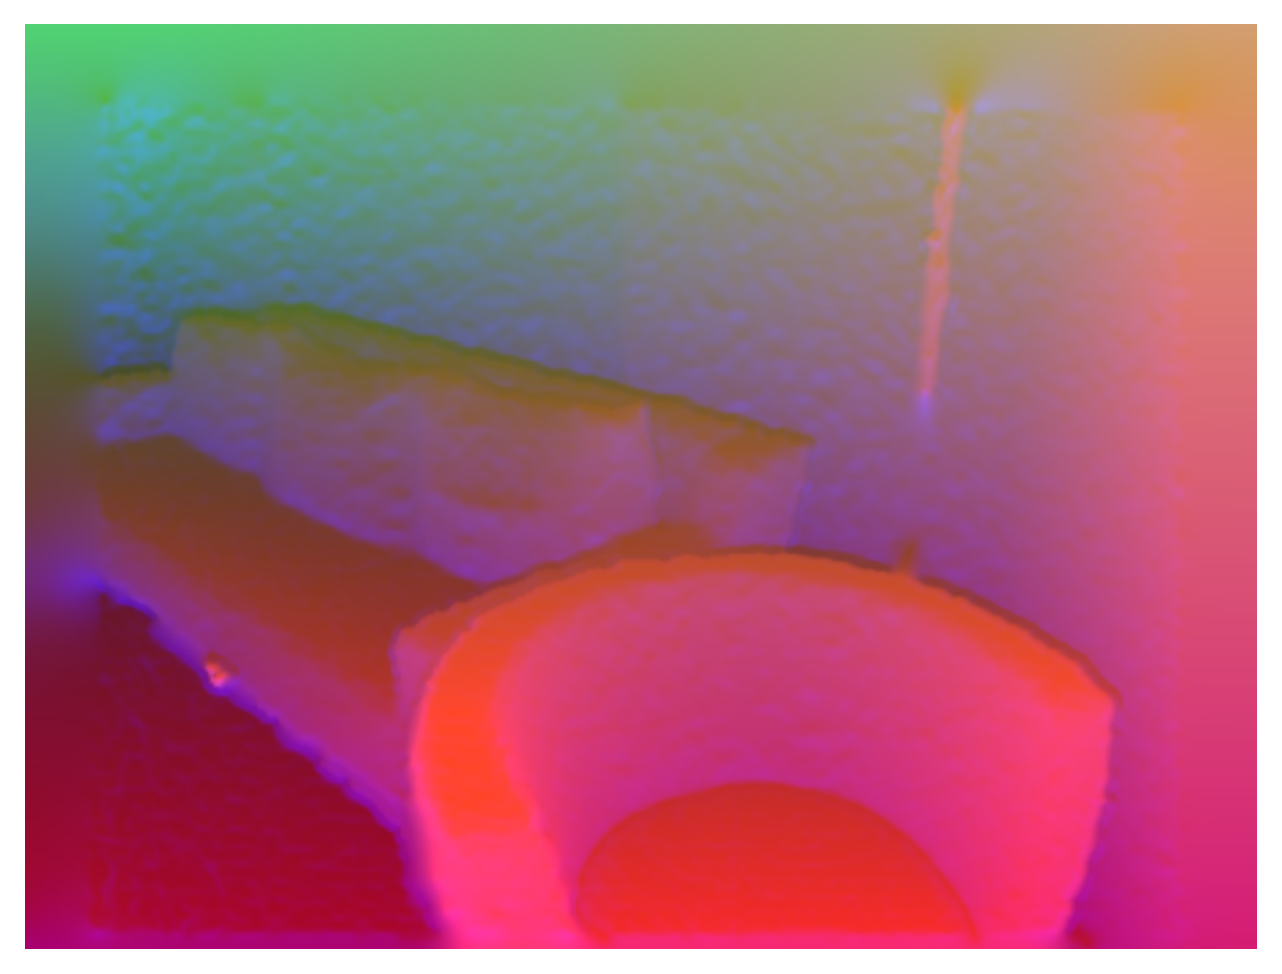}
\end{minipage}
}\hspace{-1.5mm}
\subfloat[ground truth]{
\begin{minipage}[b]{0.15\textwidth}
\centering
\includegraphics[scale=0.2]{./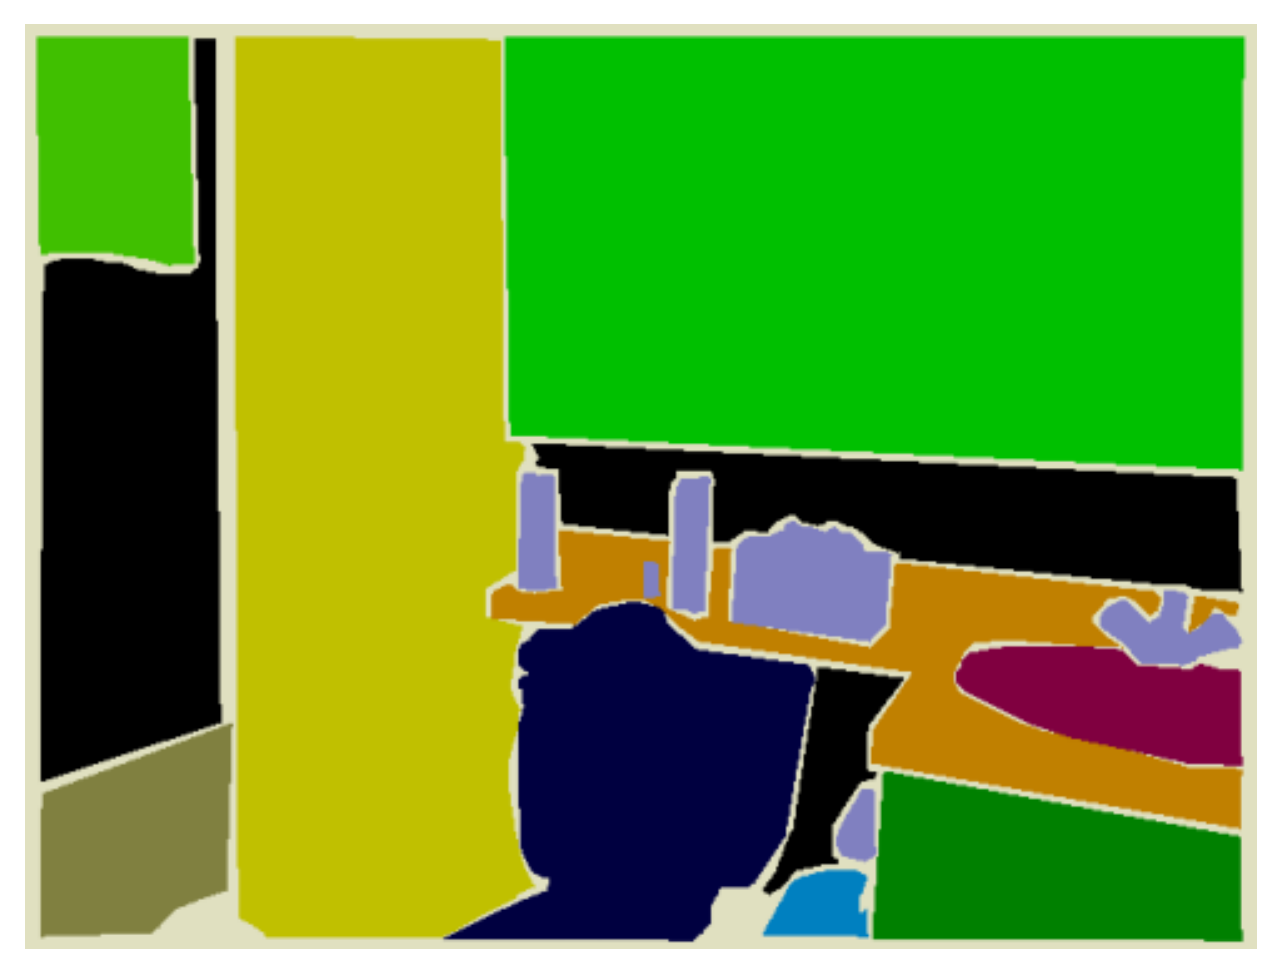} \\
\includegraphics[scale=0.2]{./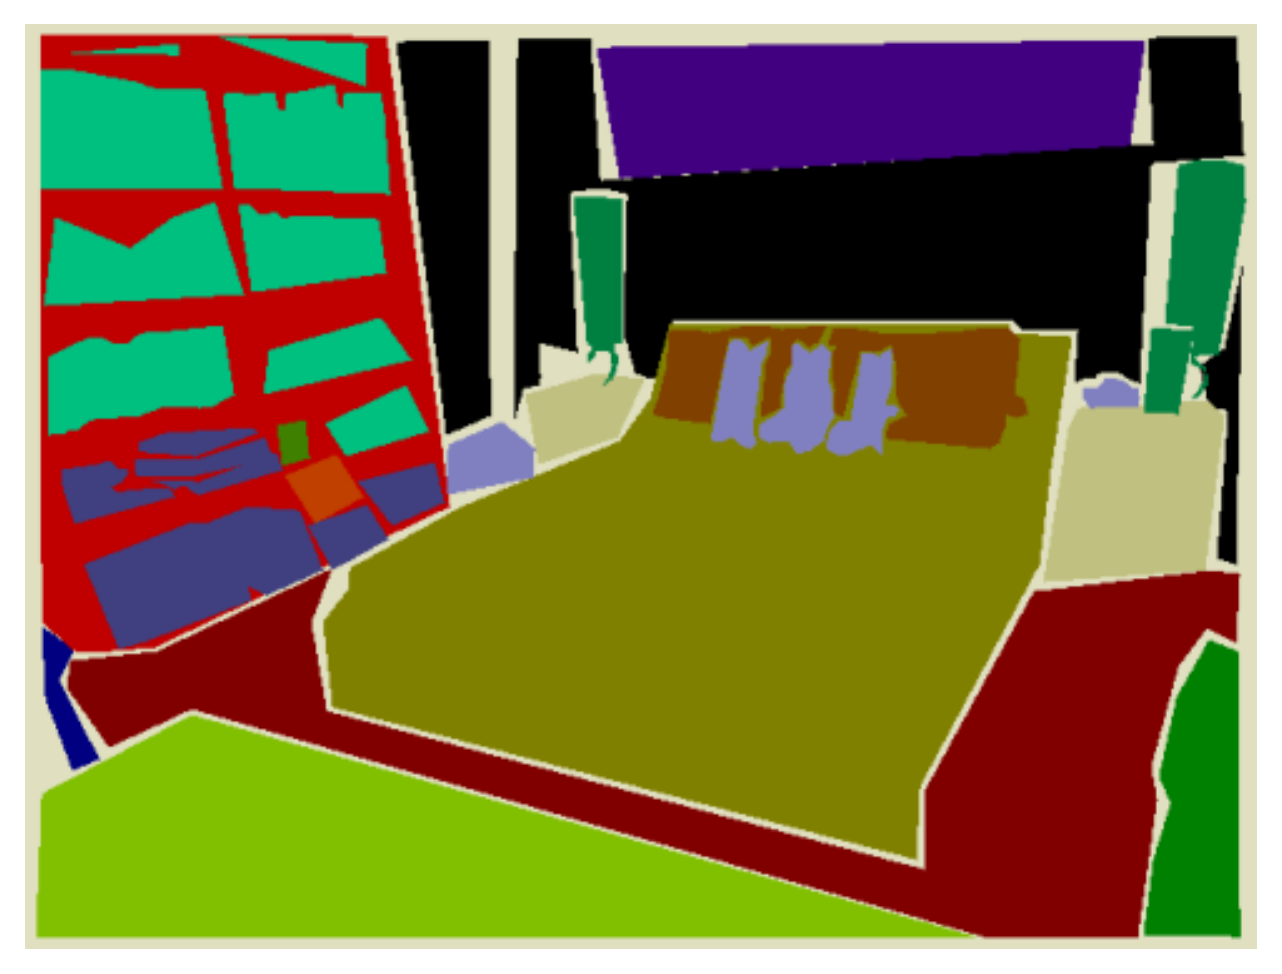} \\
\includegraphics[scale=0.2]{./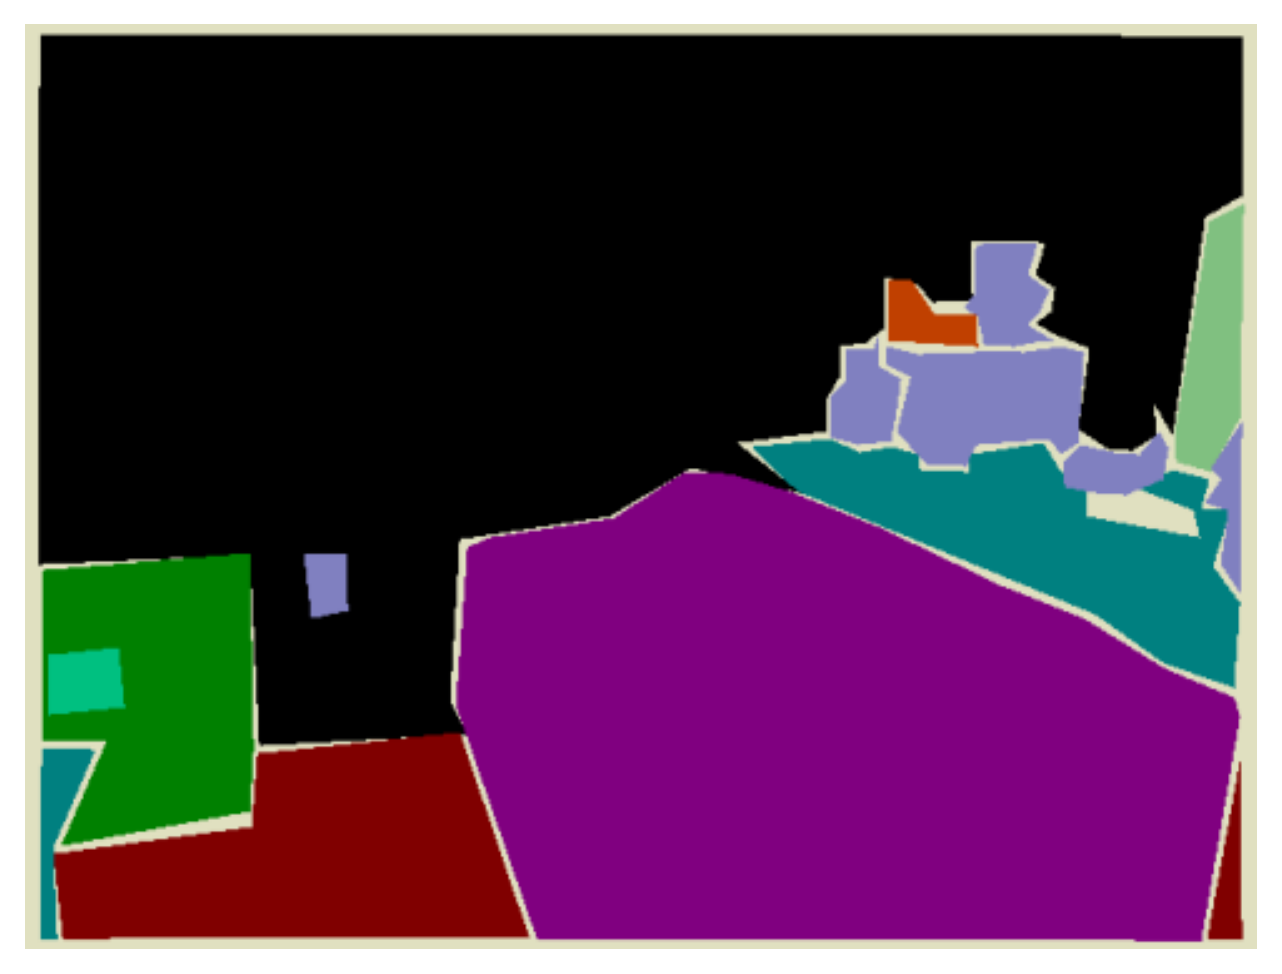} \\
\includegraphics[scale=0.2]{./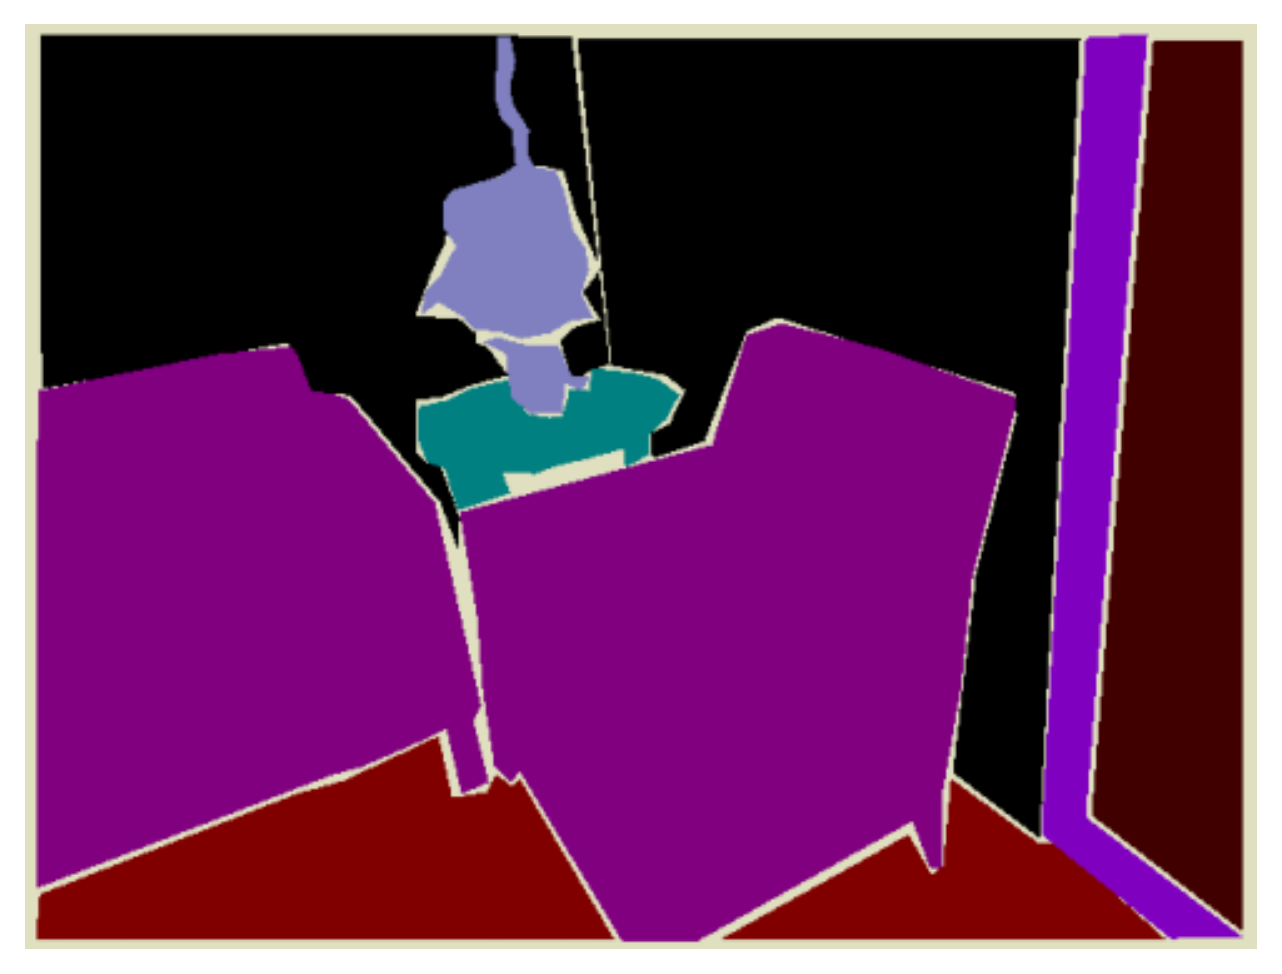} \\
\includegraphics[scale=0.2]{./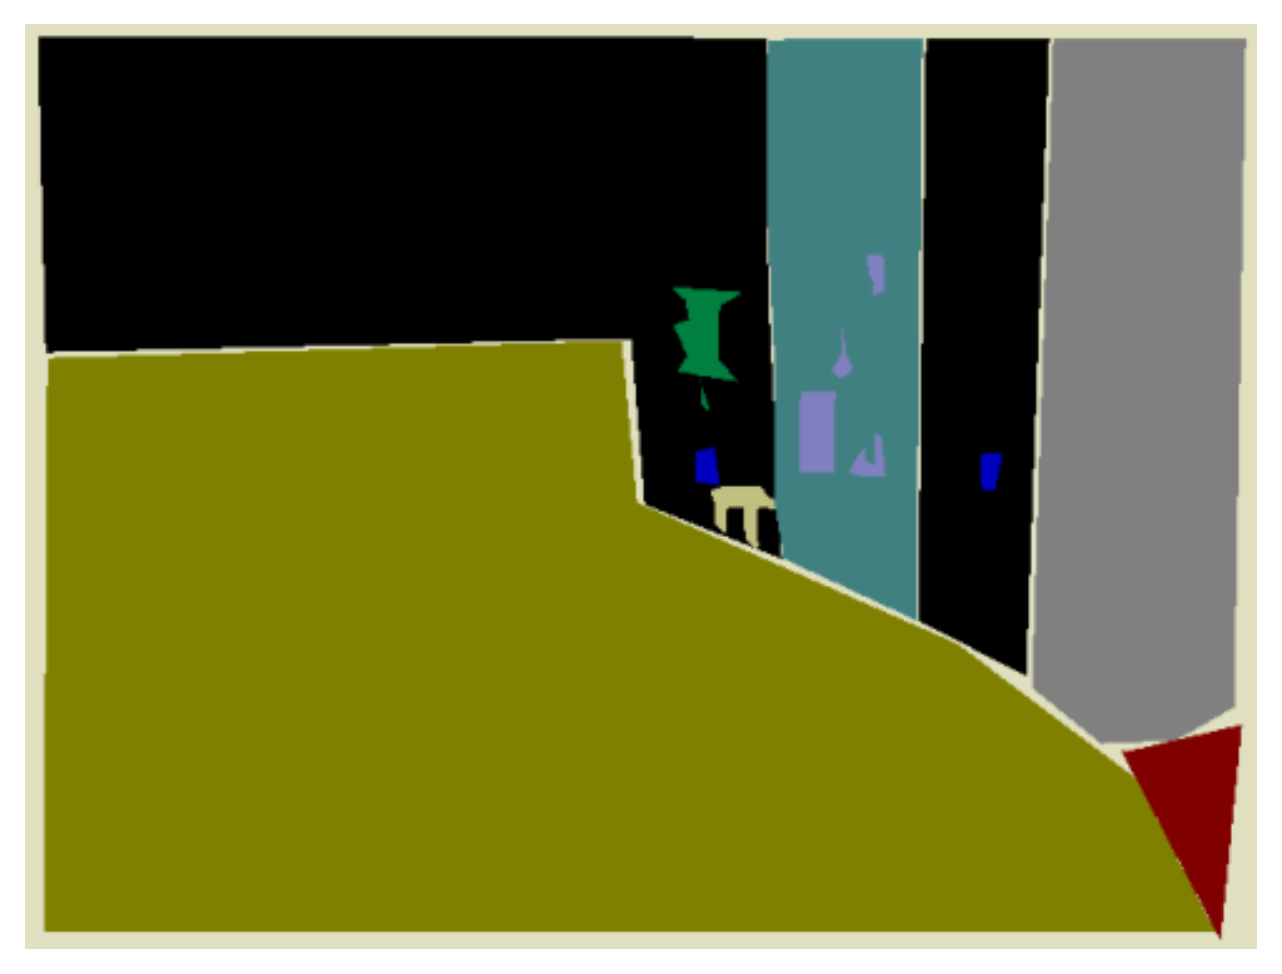} \\
\includegraphics[scale=0.2]{./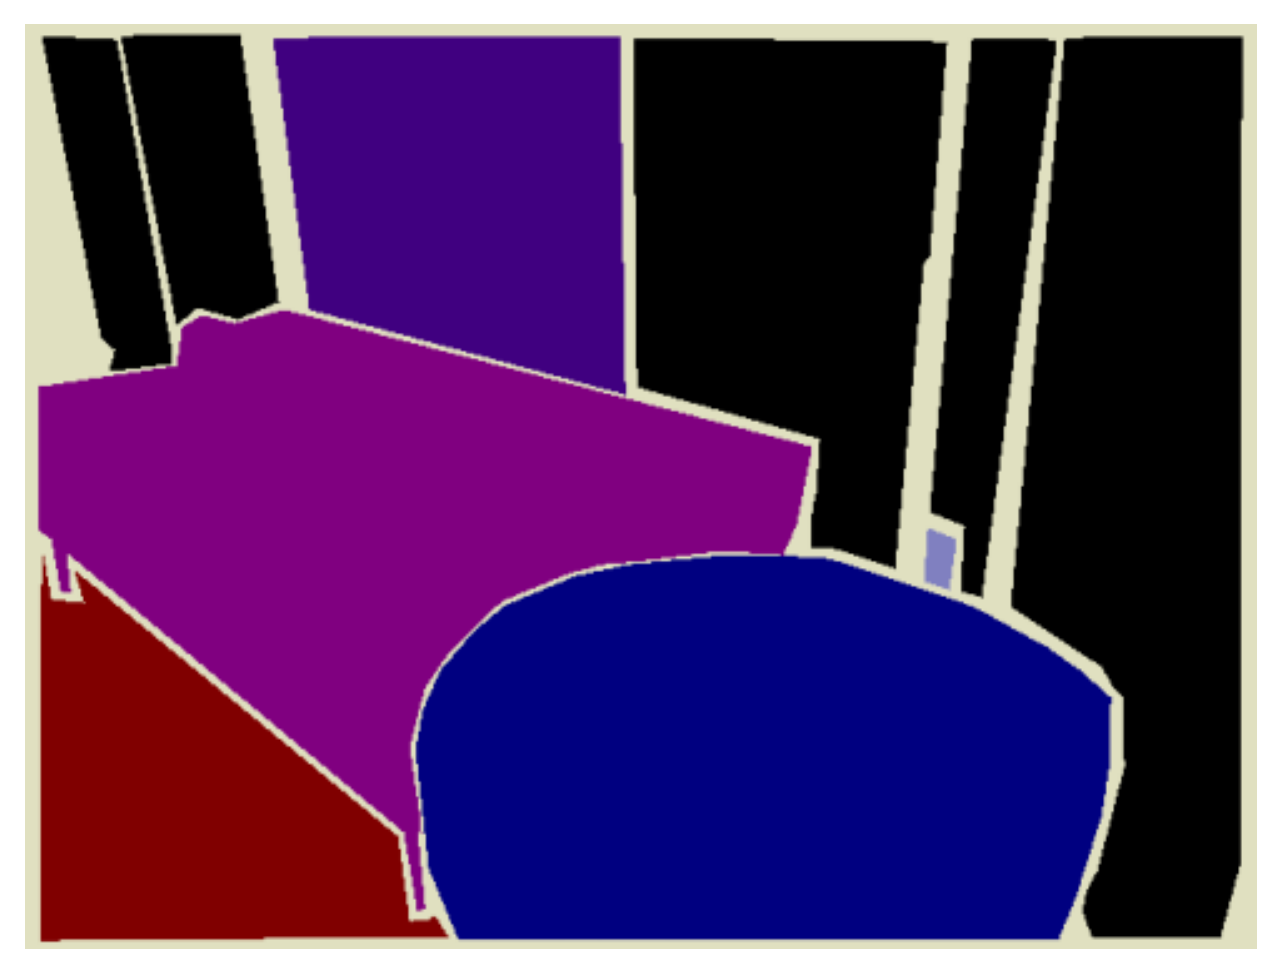} 
\end{minipage}
}\hspace{-1.5mm}
\subfloat[MM student (ours)]{
\begin{minipage}[b]{0.15\textwidth}
\centering
\includegraphics[scale=0.2]{./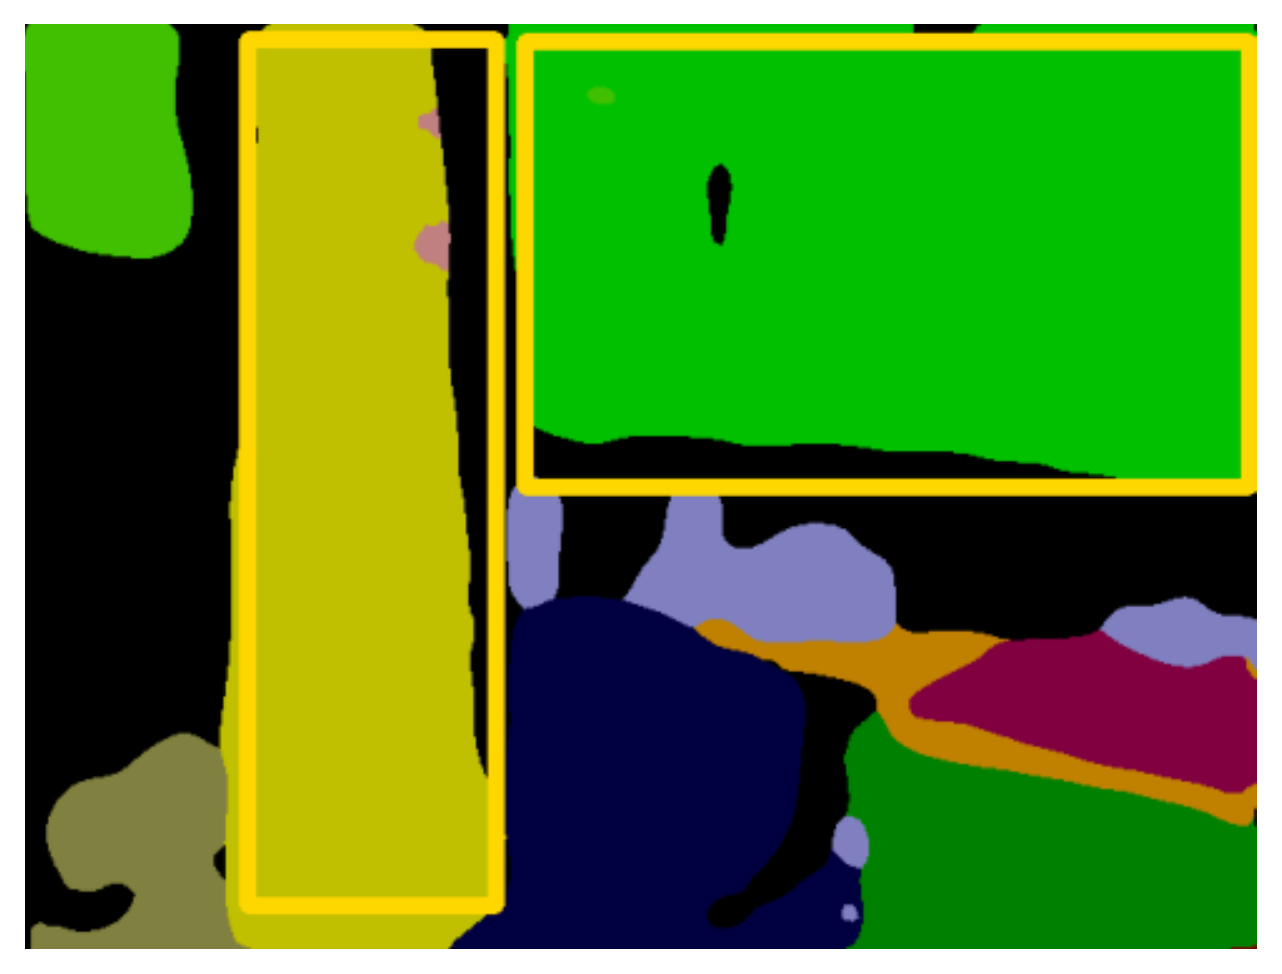} \\
\includegraphics[scale=0.2]{./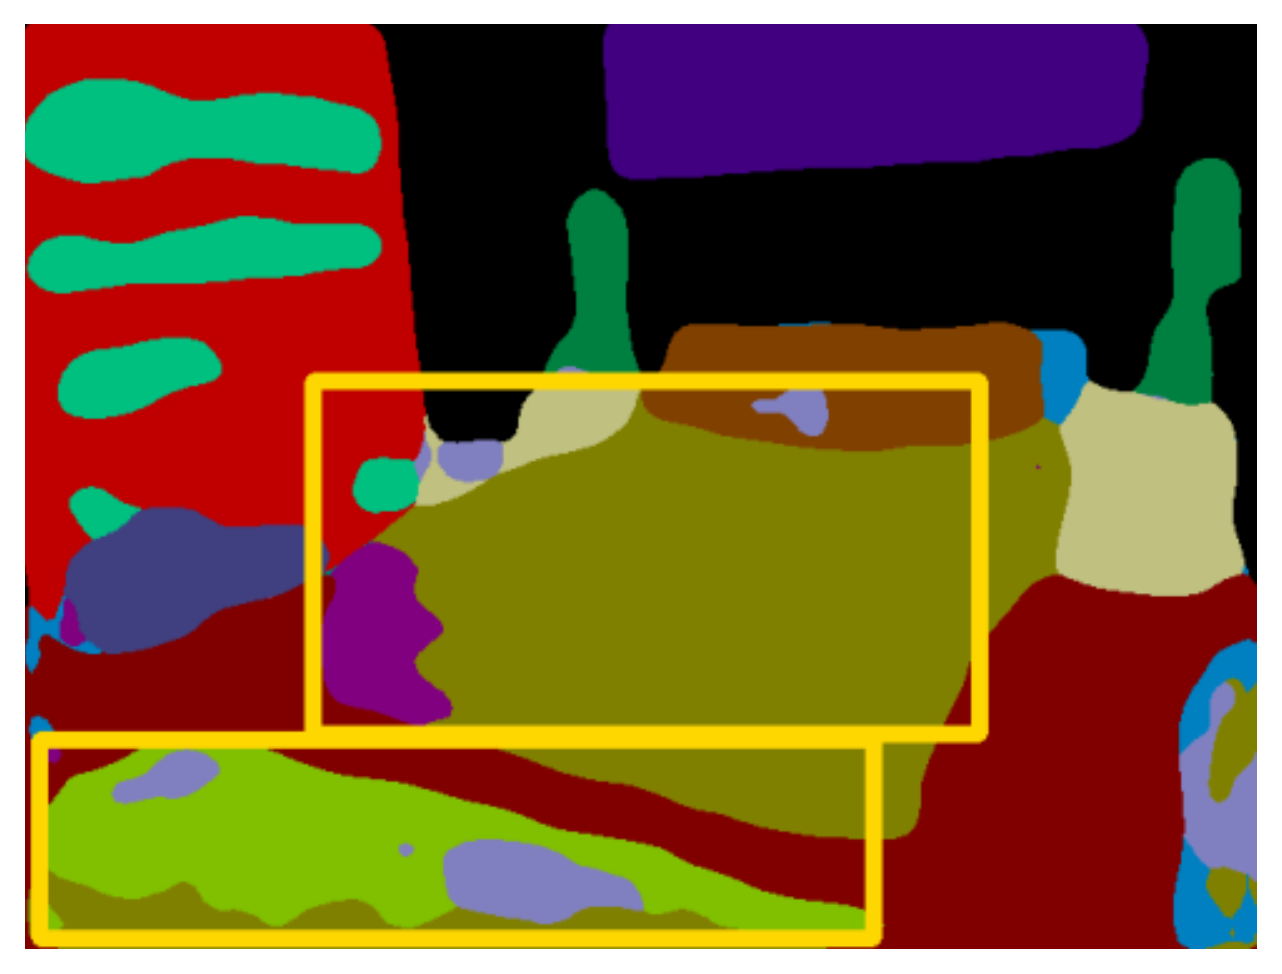} \\
\includegraphics[scale=0.2]{./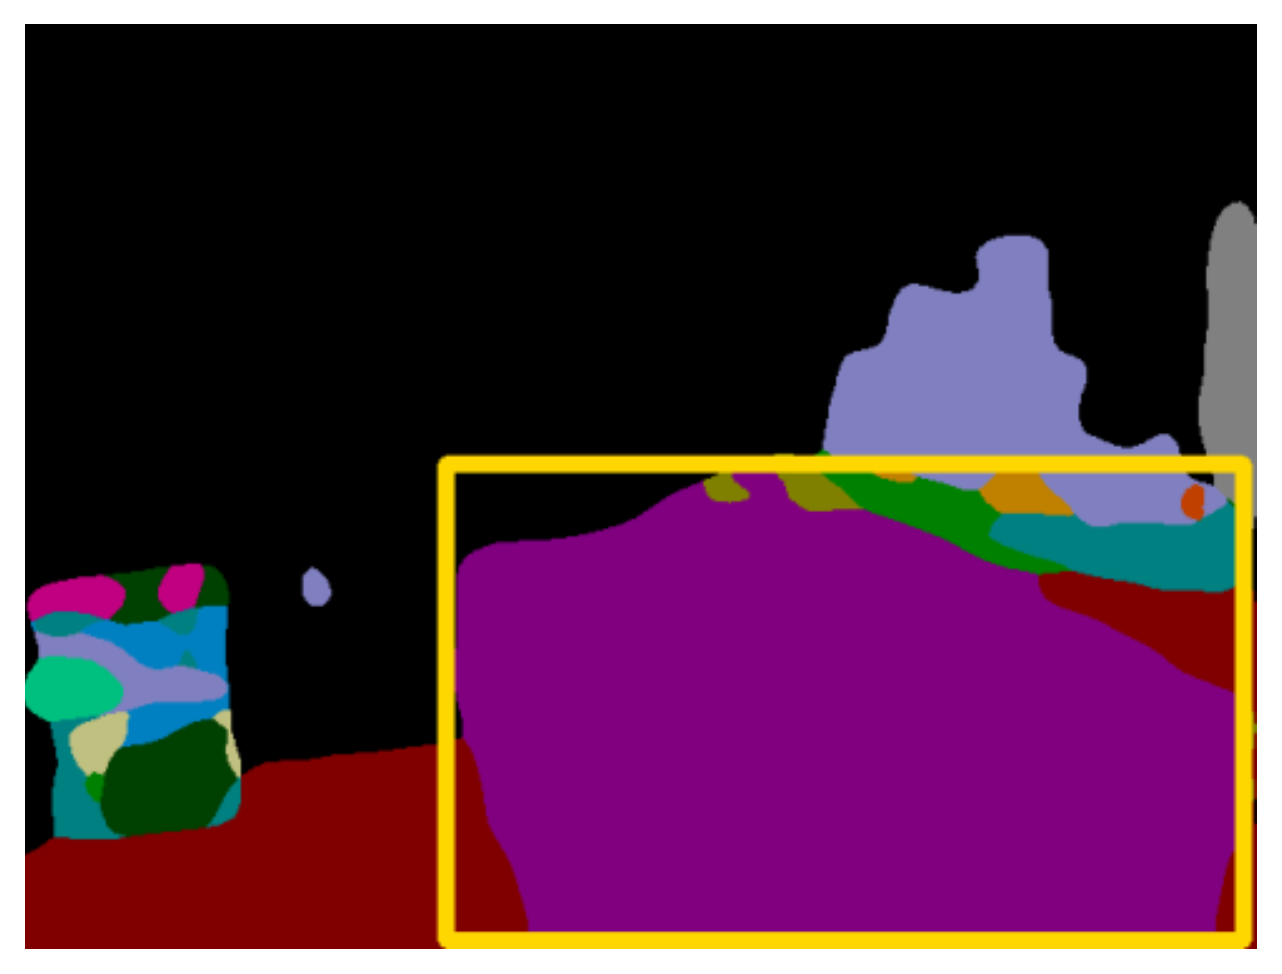} \\
\includegraphics[scale=0.2]{./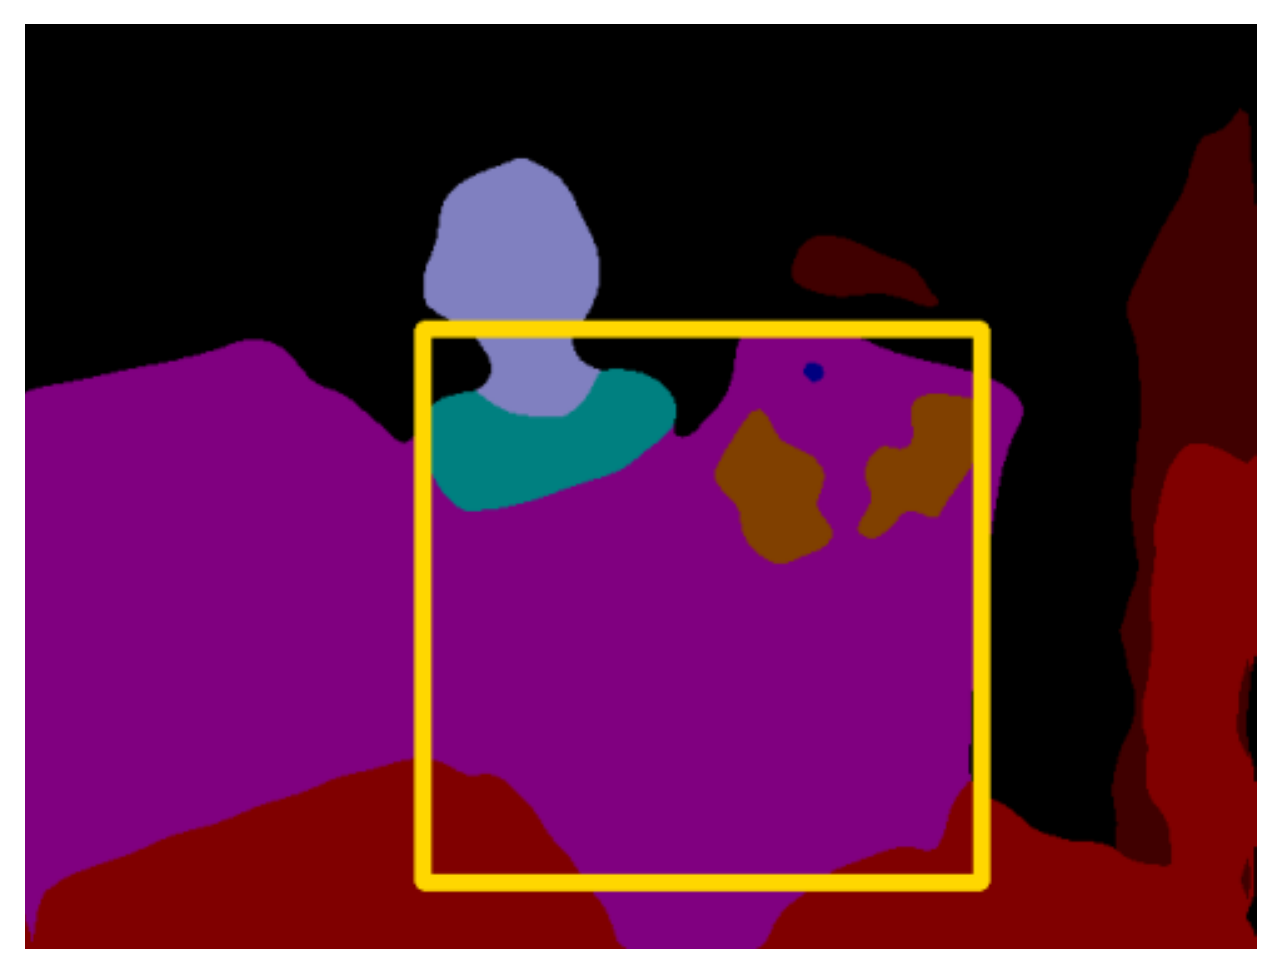} \\
\includegraphics[scale=0.2]{./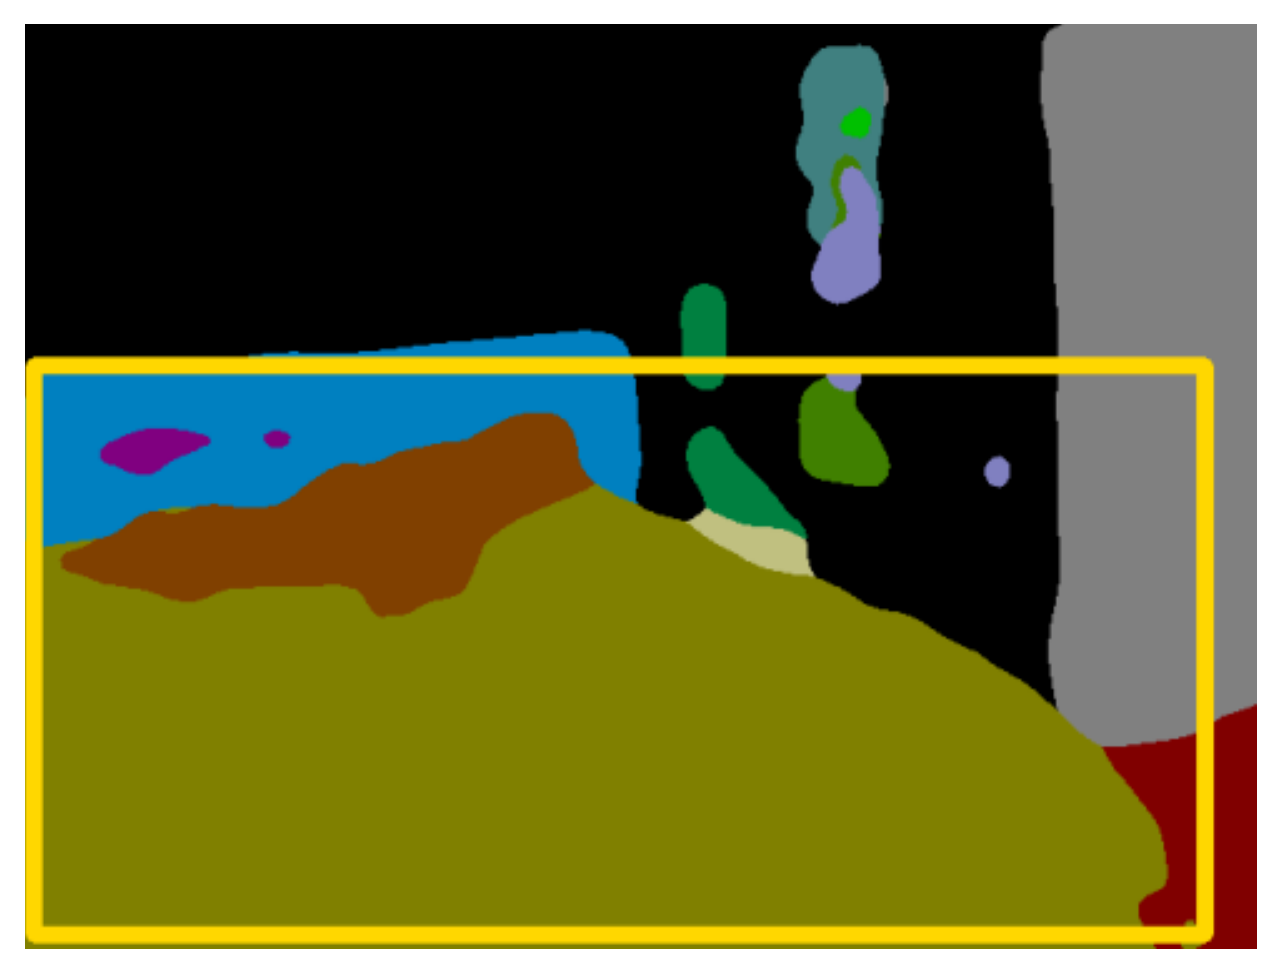} \\
\includegraphics[scale=0.2]{./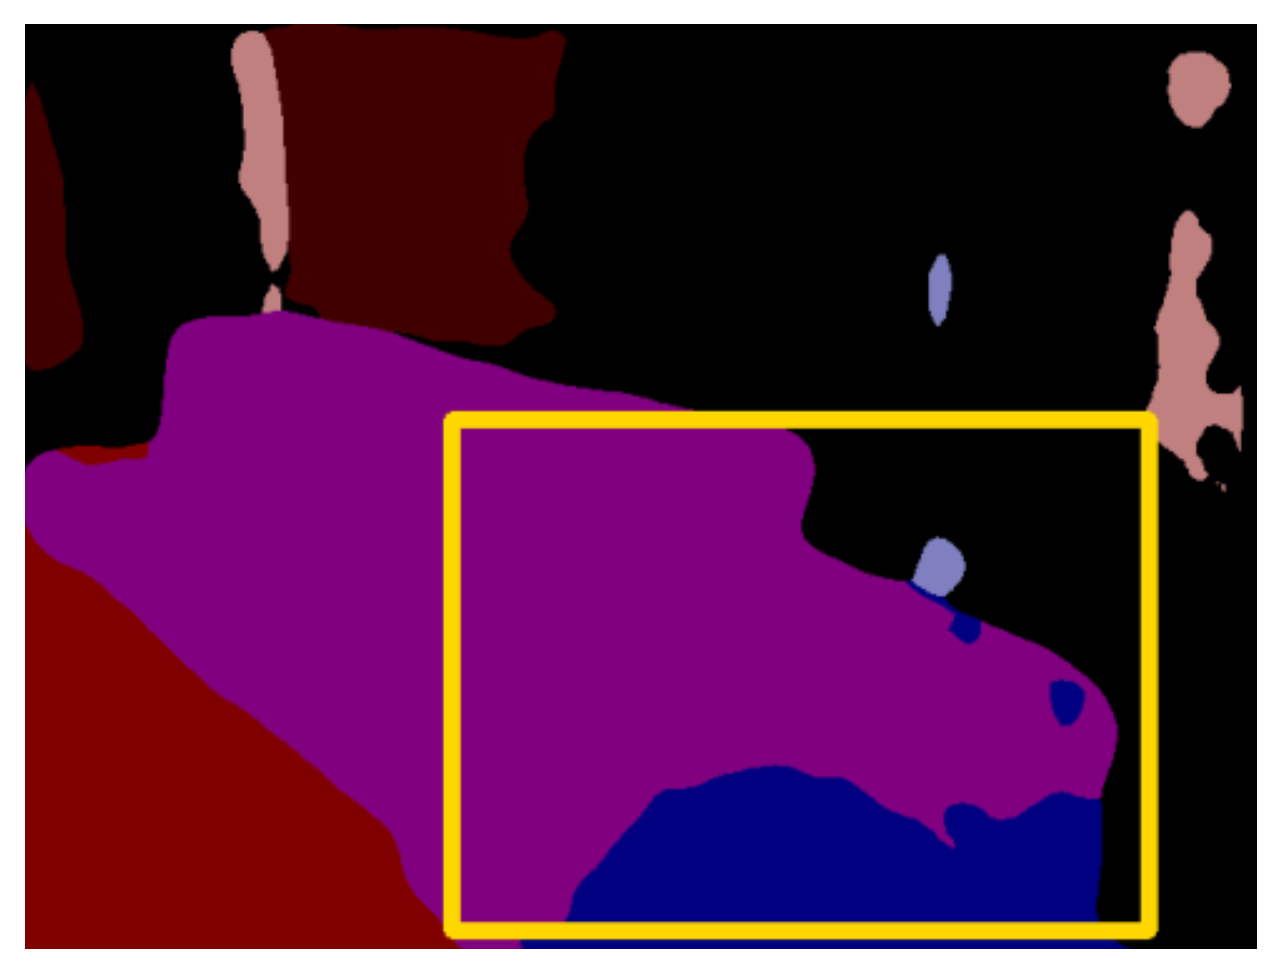}
\end{minipage}
}\hspace{-1.5mm}
\subfloat[UM teacher]{
\begin{minipage}[b]{0.15\textwidth}
\centering
\includegraphics[scale=0.2]{./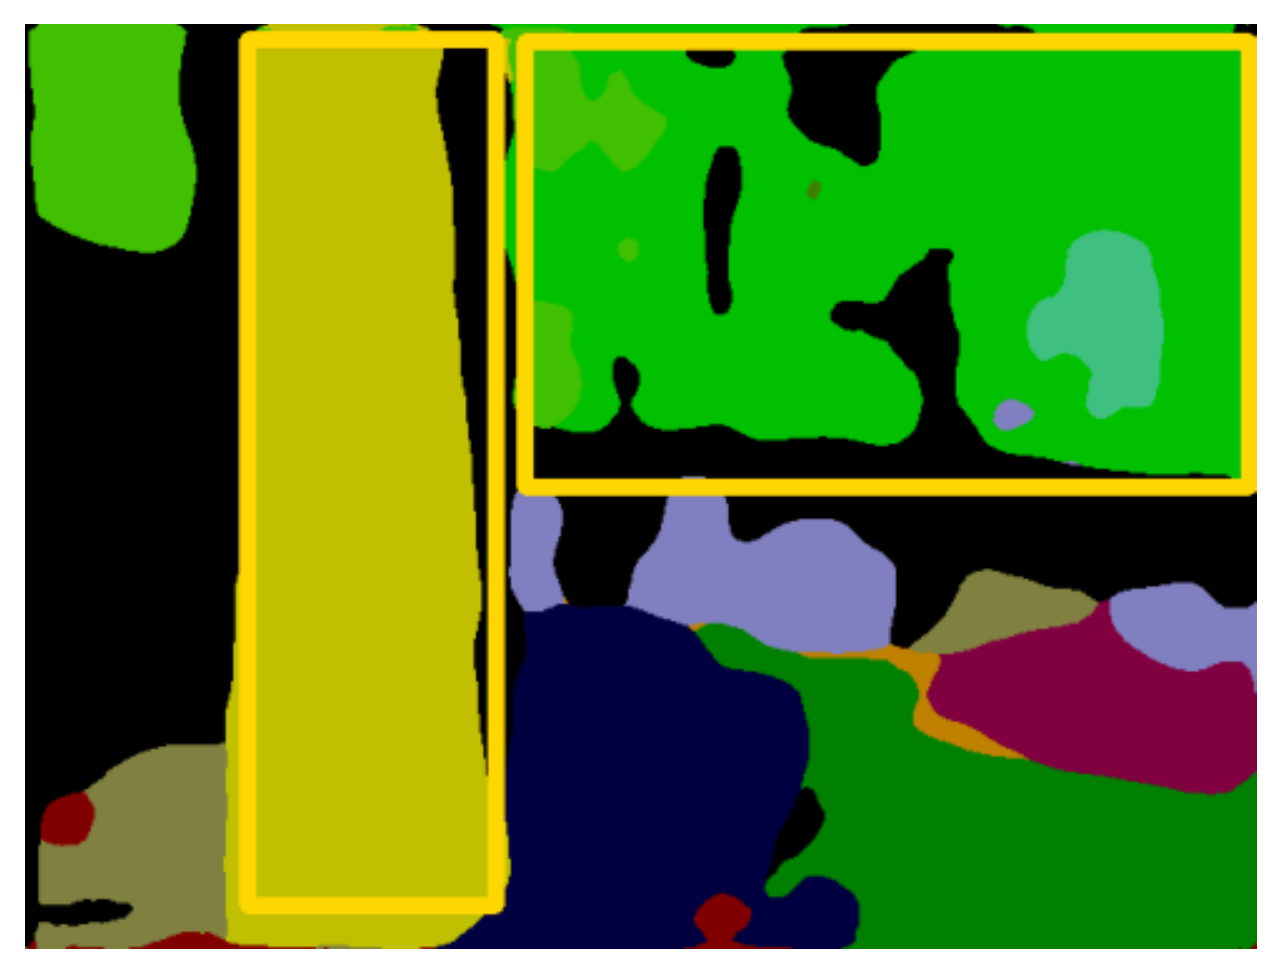} \\
\includegraphics[scale=0.2]{./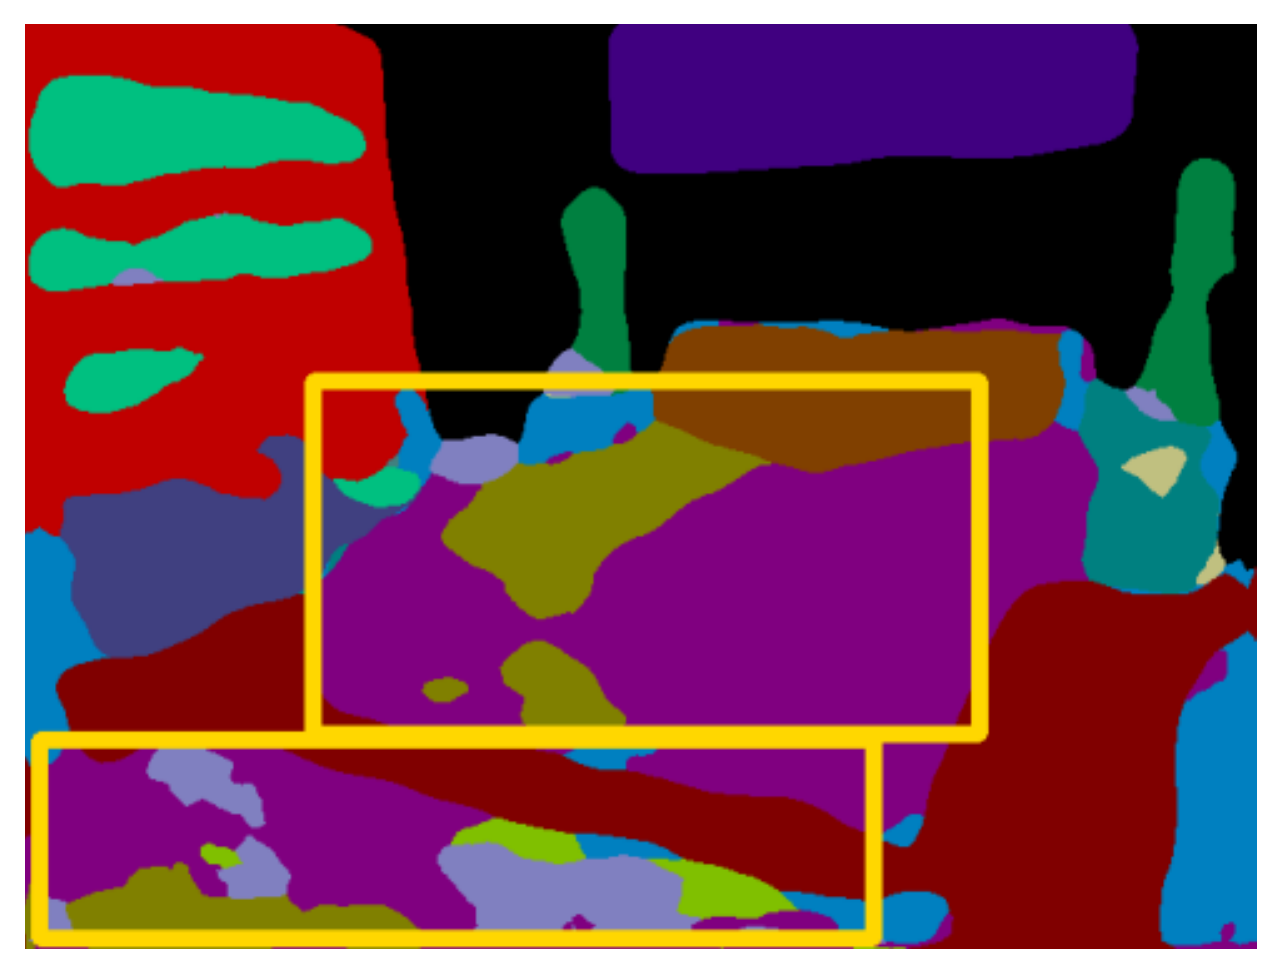} \\
\includegraphics[scale=0.2]{./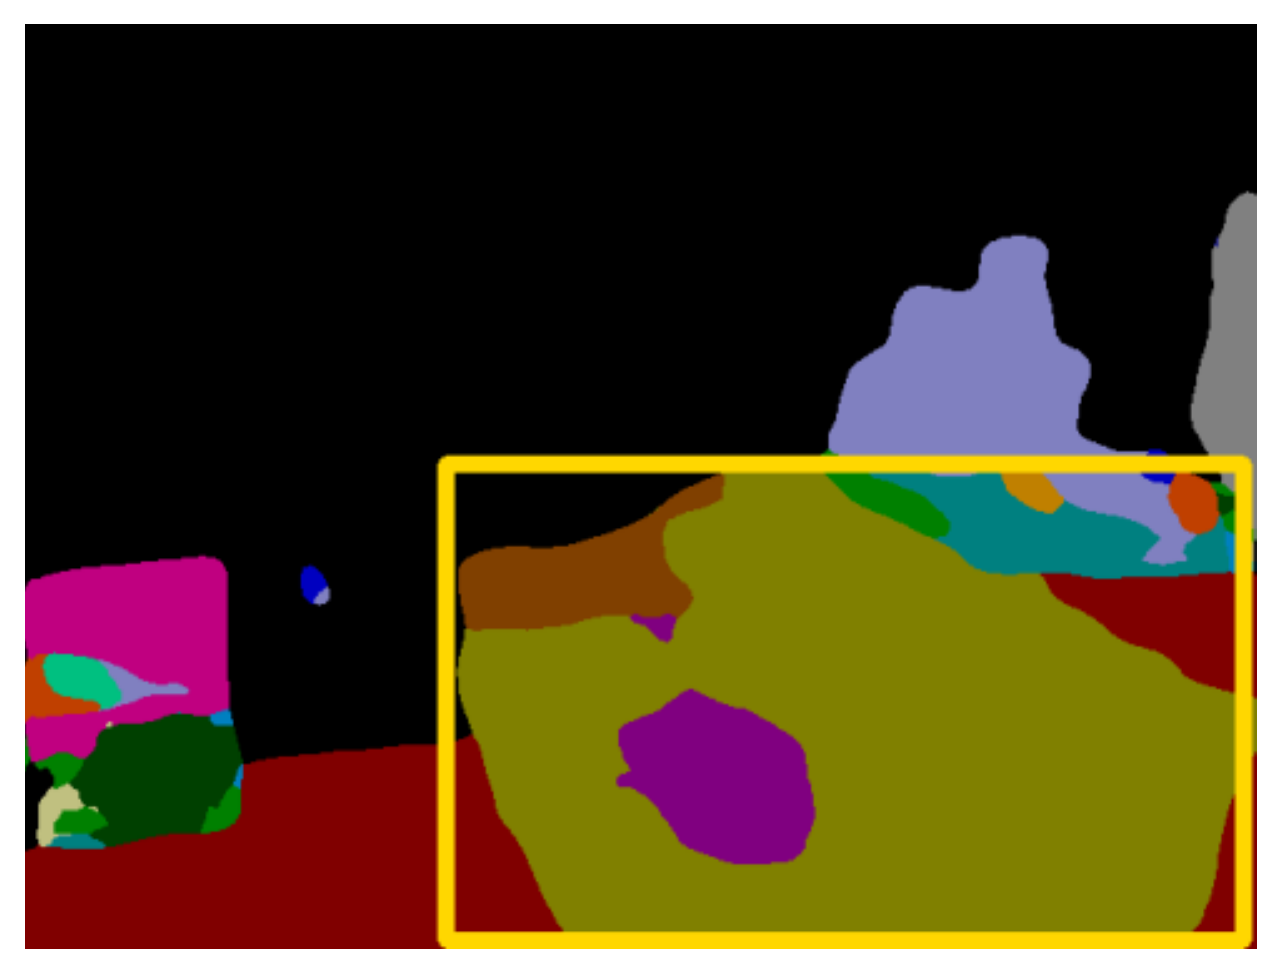} \\
\includegraphics[scale=0.2]{./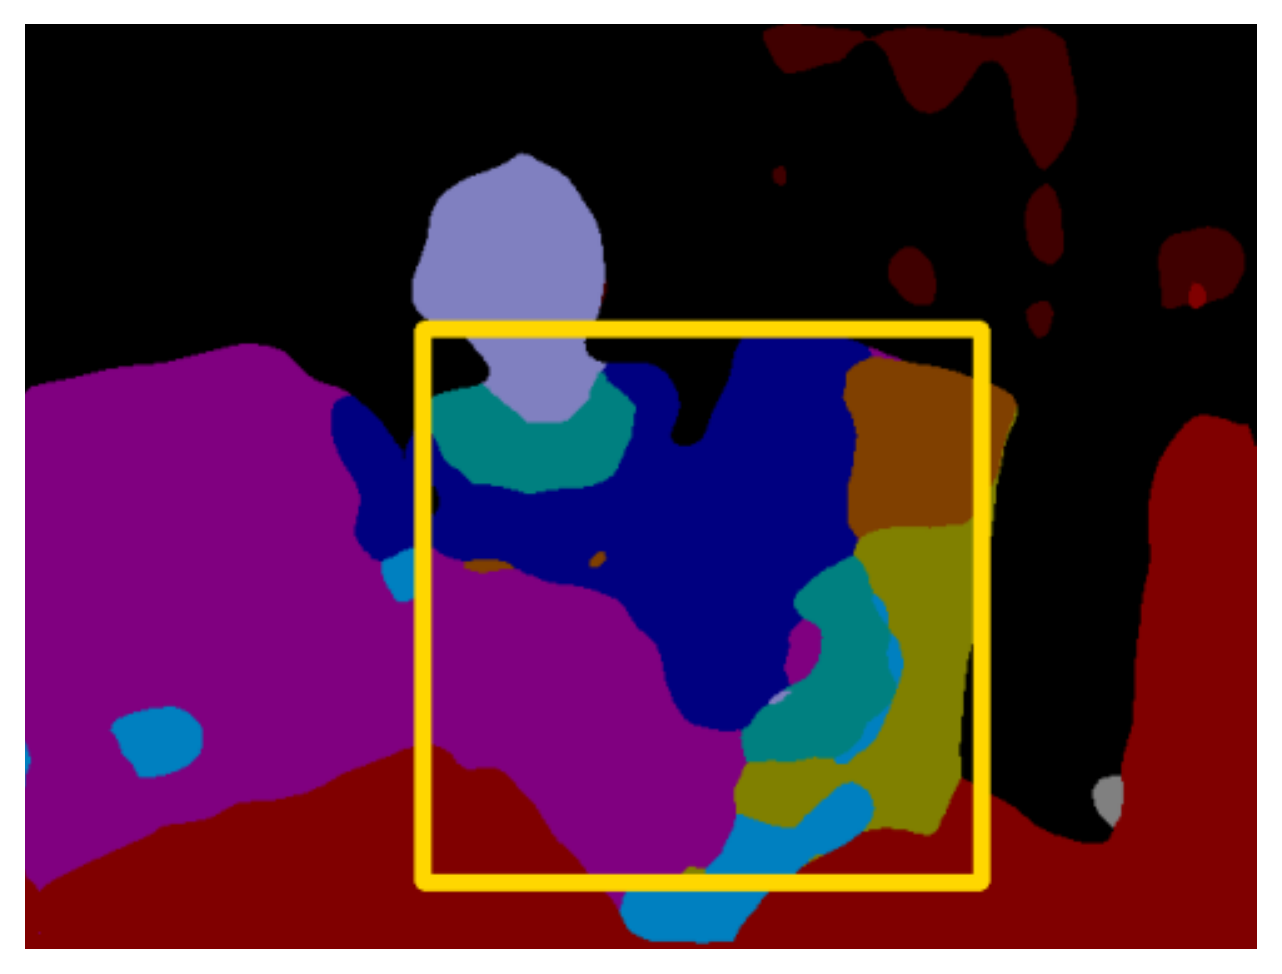} \\
\includegraphics[scale=0.2]{./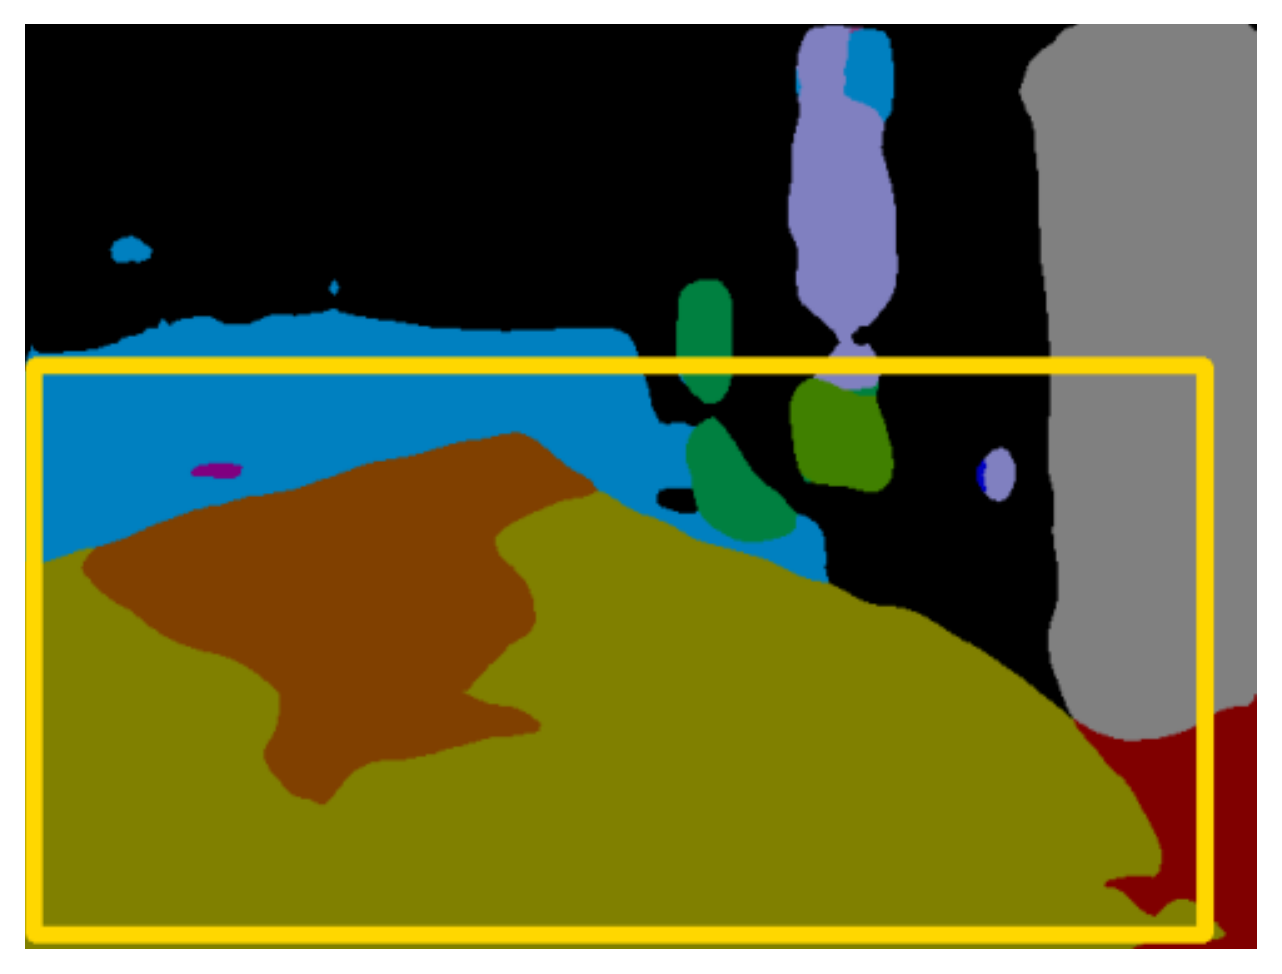} \\
\includegraphics[scale=0.2]{./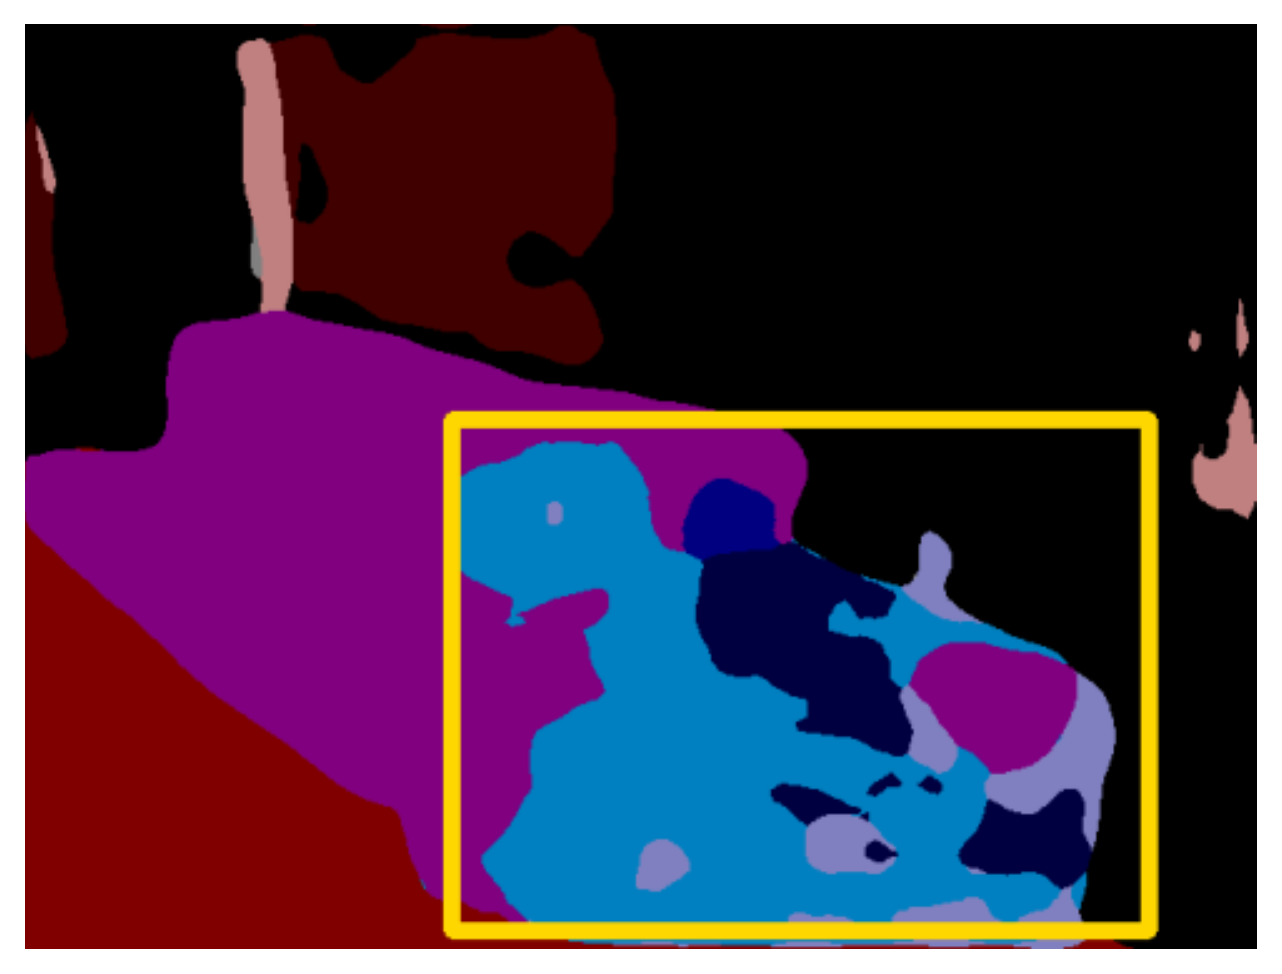} 
\end{minipage}
}\hspace{-2mm}
\subfloat[NOISY student]{
\begin{minipage}[b]{0.15\textwidth}
\centering
\includegraphics[scale=0.2]{./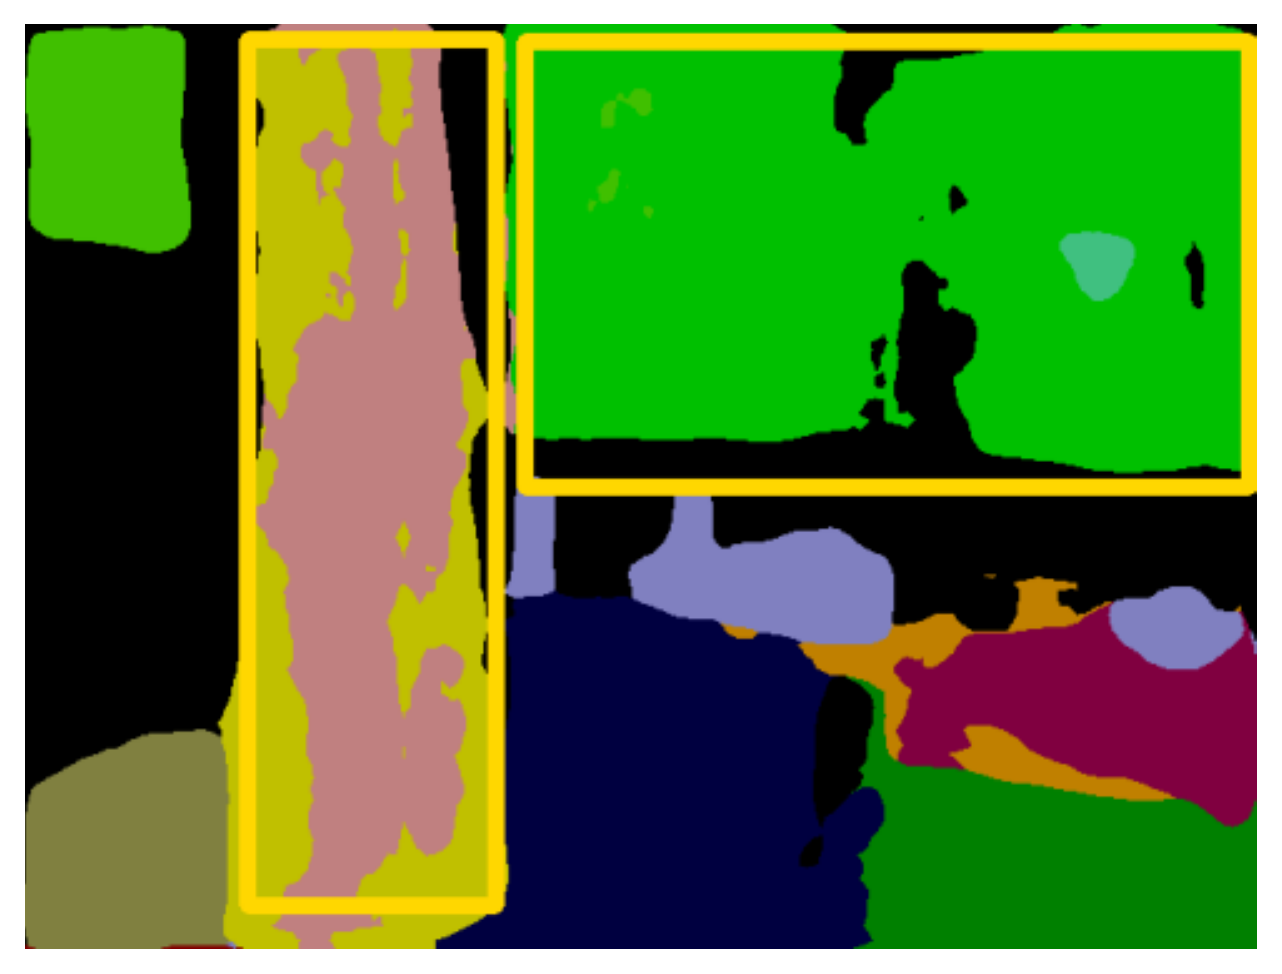} \\
\includegraphics[scale=0.2]{./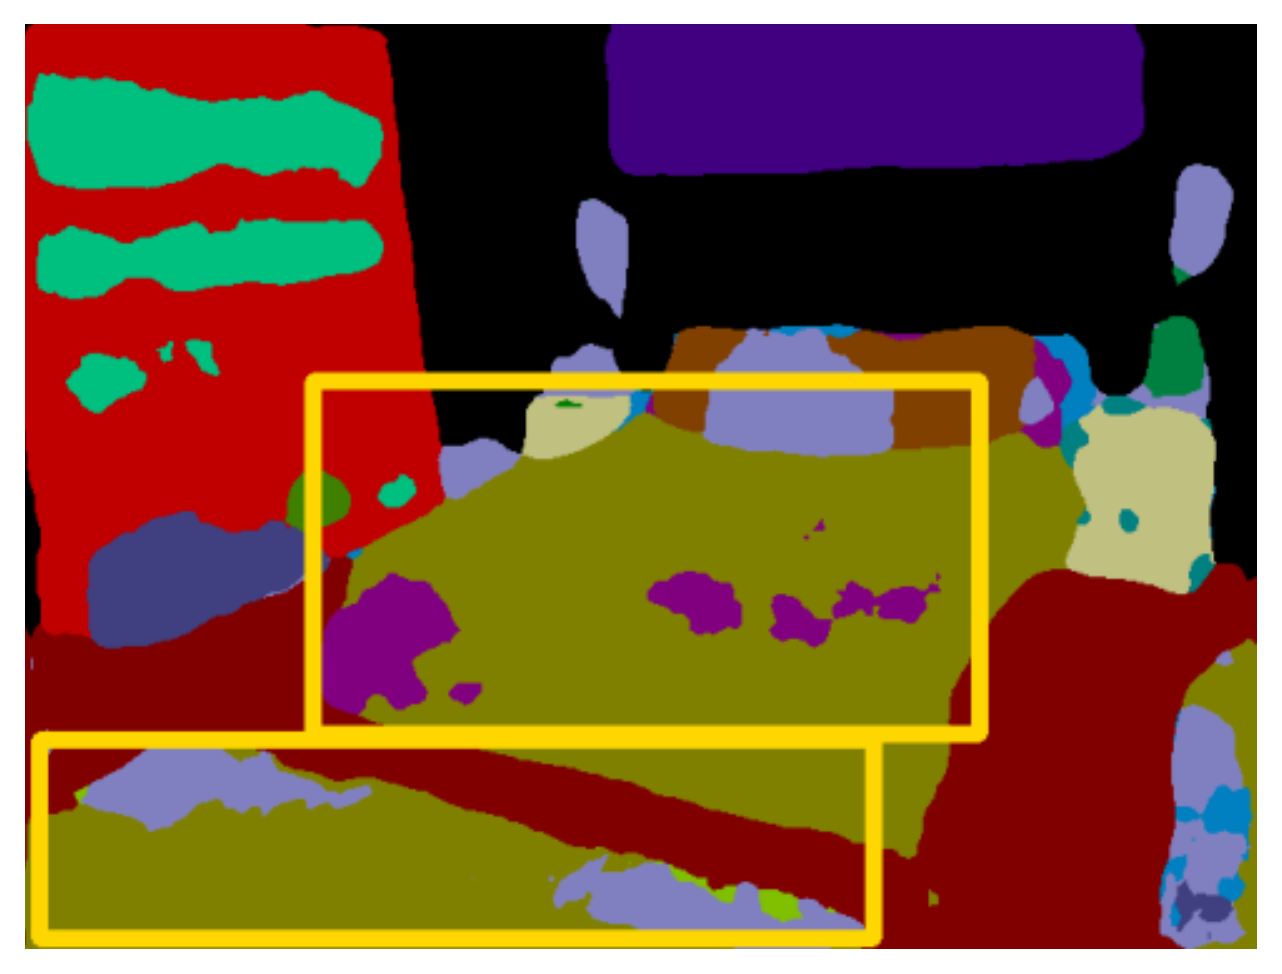} \\
\includegraphics[scale=0.2]{./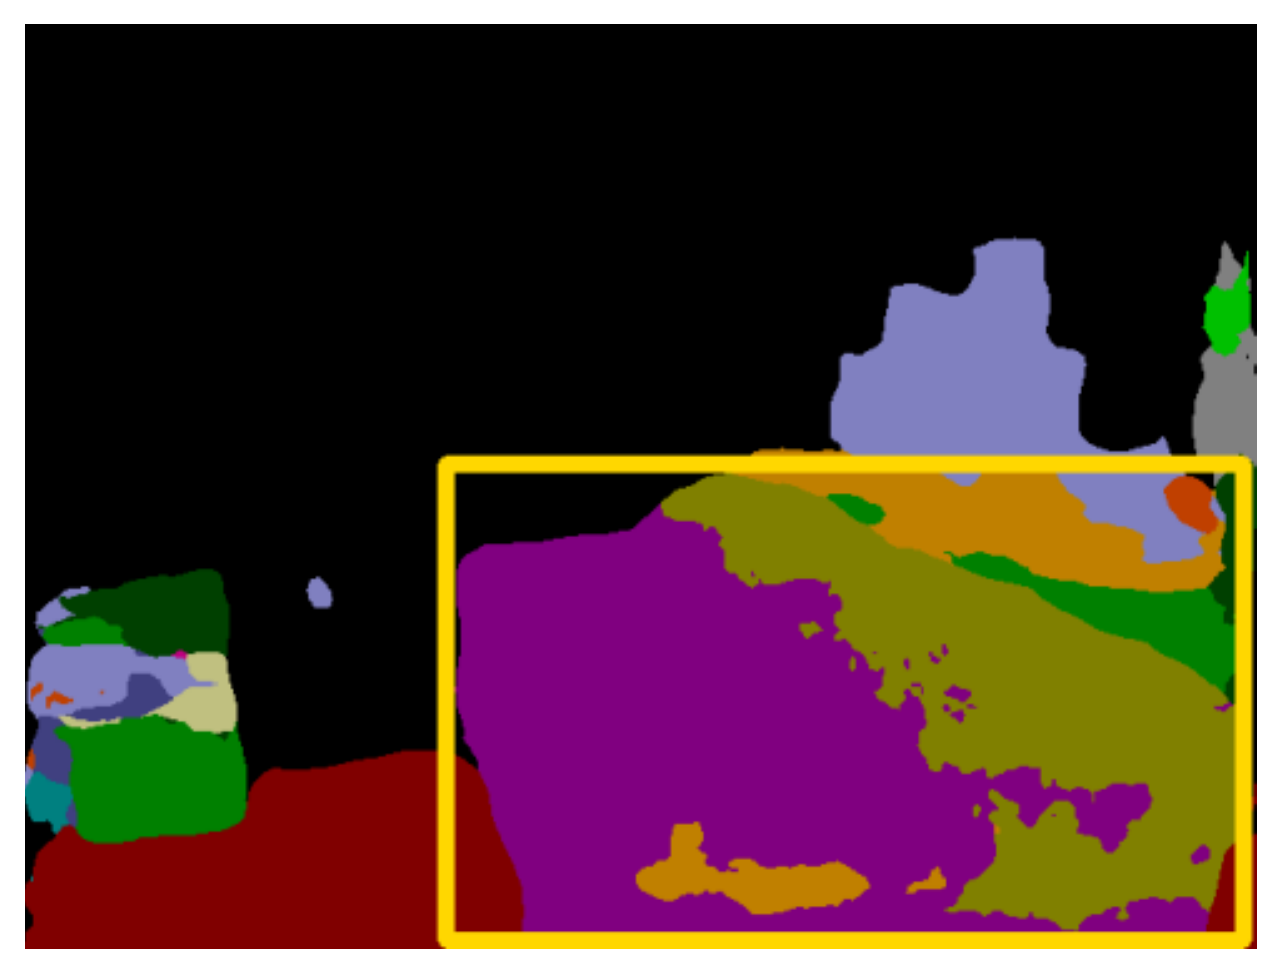} \\
\includegraphics[scale=0.2]{./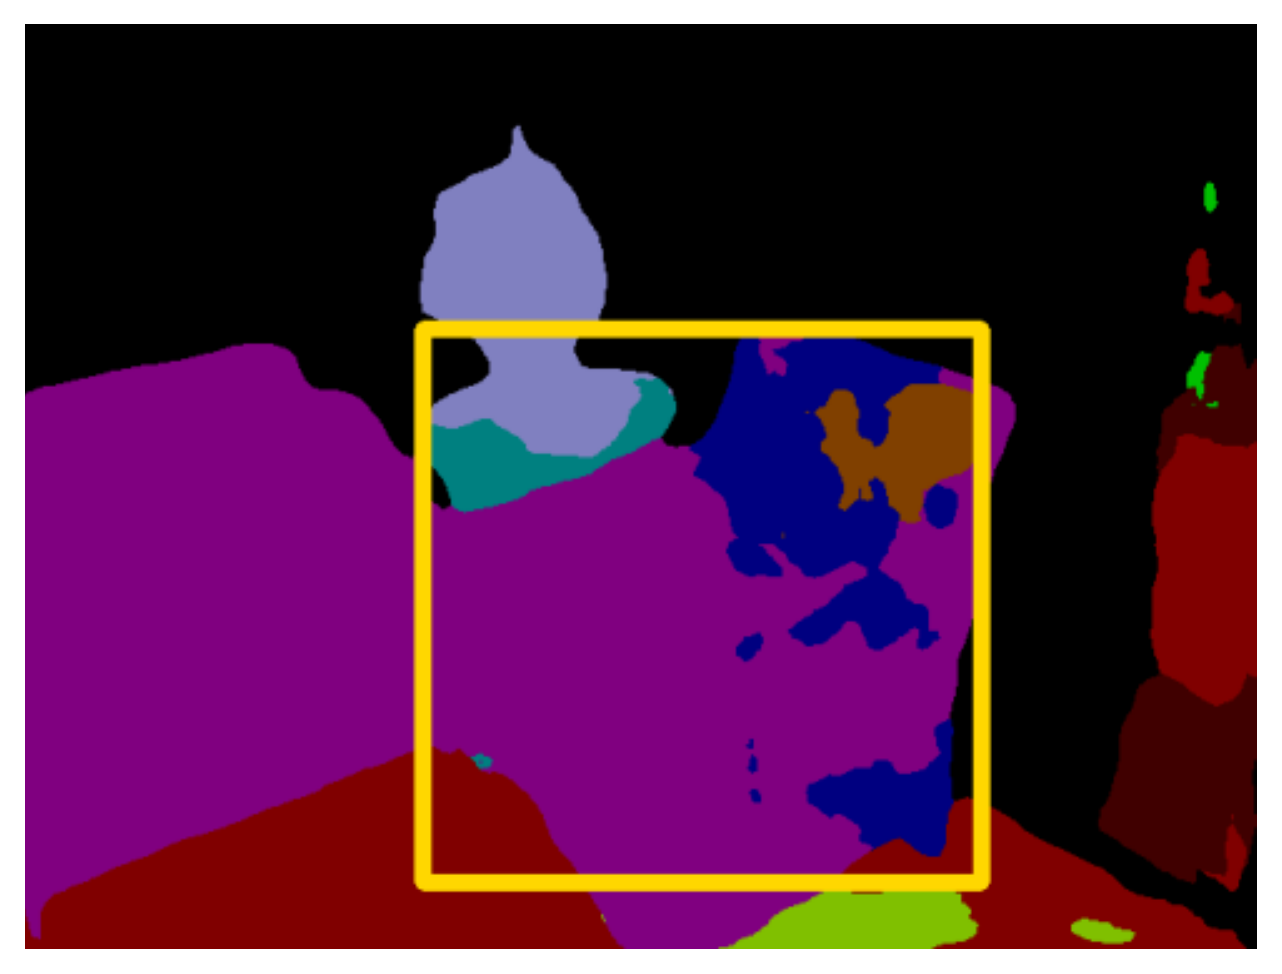} \\
\includegraphics[scale=0.2]{./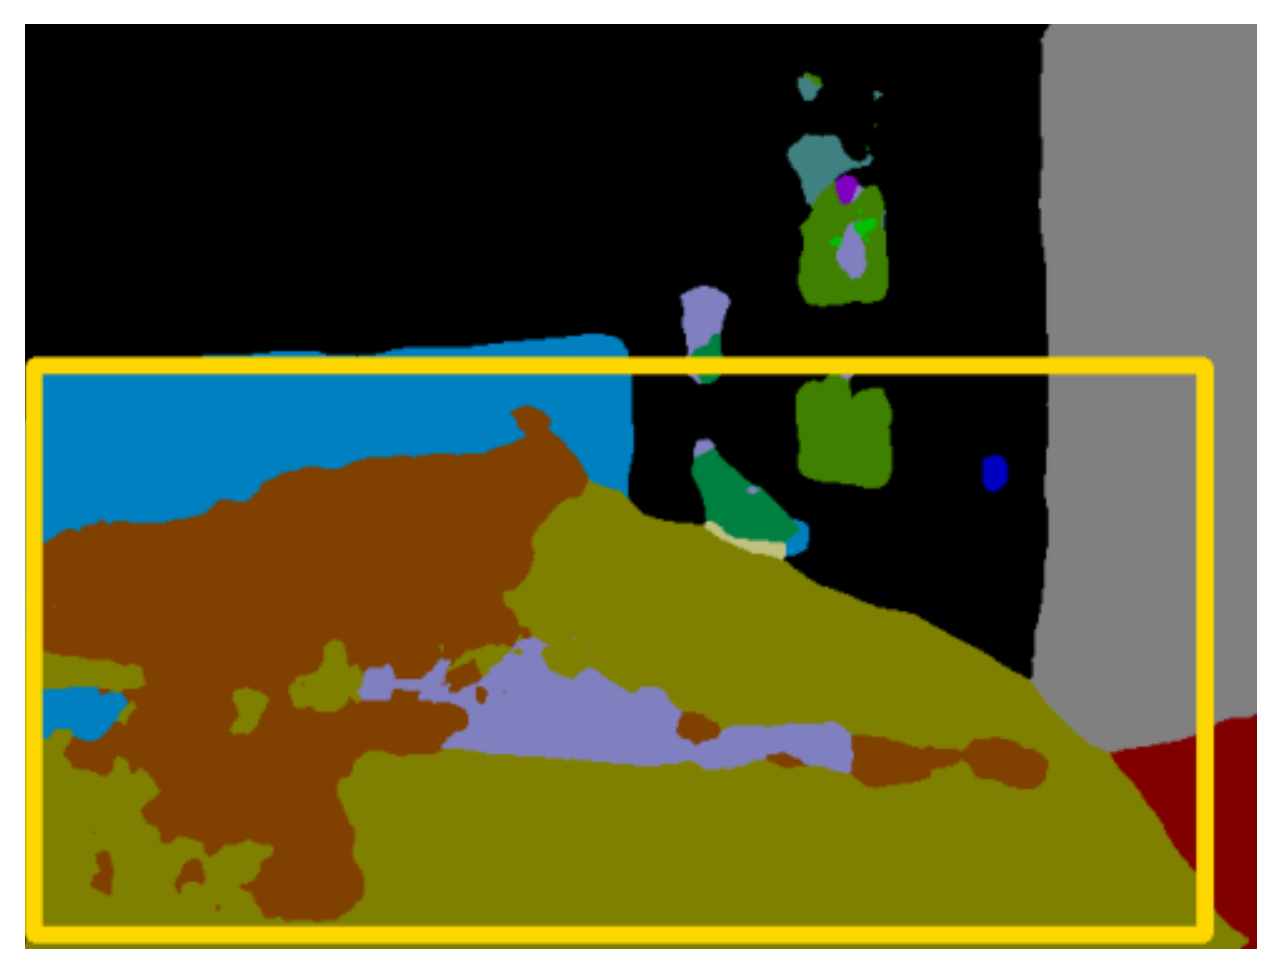} \\
\includegraphics[scale=0.2]{./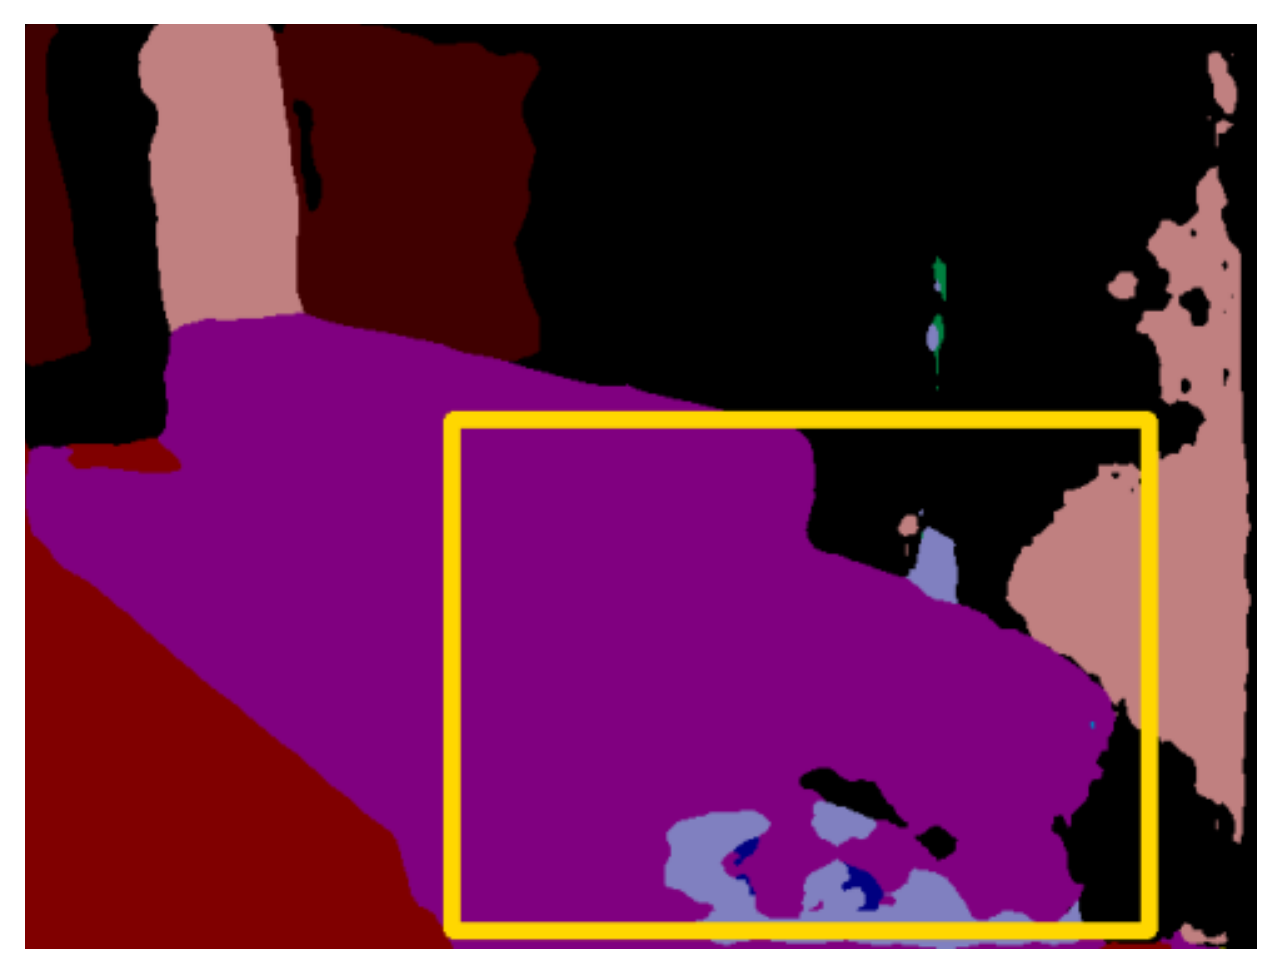} \\
\end{minipage}
}\hspace{-1.5mm}
\caption{Qualitative segmentation results on NYU Depth V2 test set.}
\label{fig:seg}
\end{figure*}

We list top 5 event categories that our MM student improves most in Table \ref{tab:eventimprove}. While NOISY student leads to similar performance gain for each event class, our MM student greatly improves over these classes with the assistance of video modality. For instance, the UM teacher performs poorly on the ``dog growling'' class with audio inputs only. NOISY student improves test mAP from 0.069 to 0.096 with the help of more data. In contrast, a MM student achieves an mAP of 0.542 and shows great improvement over the unimodal baselines. Video modality helps our MM student denoise these incorrect predictions given by the UM teacher.
