# Supplementary material for: Multimodal Knowledge Expansion
Source: arXiv:2103.14431 source file (2021-10-29)
Supplement: Supplementary file 2 [file supp3-ablation.tex]

\section{Ablation Studies}
In this section, we provide a comprehensive study of various factors in \textit{MKE}. 
\subsection{Regularization}
The ablation study for regularization terms is provided in the main paper. We report performance of MM student (no reg), \ie, a MM student without regularization in all experiments. Results consistently show that a MM student yields better results than a MM student (no reg). We arrive at the conclusion that multimodality combined with regularization leads to best performance compared with all the baselines.

\subsection{Unlabeled Data Size}
We study the effect of unlabeled data size in this section. Specifically, for the task of semantic segmentation, we reduce unlabeled data size from 1488 RGB-D image pairs as reported in the main paper to 744 image pairs. Results are shown in Table \ref{tab:seg}.

\begin{table}[H]
\centering
\begin{tabular}{ccccc}
\toprule
\multirow{2}*{Method} & \multicolumn{3}{c}{Train data} & \multirow{2}*{\makecell[c]{Test mIoU \\(\%)}} \\
~ & \textit{mod} & $D_l$ & $\tilde{D}_u$ &  ~ \\
\midrule
UM teacher & $rgb$ & $\checkmark$ & & 44.15  \\
UM student & $rgb$ &  &$\checkmark$  & 44.57  \\
NOISY student & $rgb$ & $\checkmark$ & $\checkmark$ & 46.85  \\
\makecell[c]{MM student (ours)}& $rgb, d$ & & $\checkmark$ & \textbf{47.44}  \\
\bottomrule
\end{tabular}
\caption{Results of semantic segmentation on NYU Depth V2. We set unlabeled data size smaller than labeled data size.}
\label{tab:seg}
\end{table}

UM student yields marginal improvement over UM teacher as it receives a small amount of unlabeled data and pseudo labels for training. On the contrary, provided with same data as the UM student, a MM student still achieves a mIoU gain of 3.29\%. Furthermore, although training data of NOISY student is twice greater than that of a MM student, half of which contain true labels, our MM student still achieves better results with respect to NOISY student. The great denoising capability of \textit{MKE} is thus shown.

\subsection{Teacher Model}
The UM teacher of previous experiments on NYU Depth V2 is implemented as DeepLab V3+. In this section, we experiment with the teacher model as RefineNet. We utilize same data as in Section 4.2, where $|D_l|=795$, $|D_u|=744$, and $|D_{test}|=654$. Table \ref{tab:ablation-teacher} reports performance when the UM teacher is RefineNet with ResNet-50 and ResNet-101 as backbone respectively.

\begin{table}[H]
\centering
\begin{tabular}{cccc}
\toprule
\multirow{2}*{Method} & \multirow{2}*{\textit{mod}} & \multicolumn{2}{c}{Test mIoU(\%)} \\
~&~& \makecell[c]{RefineNet-\\Res50}& \makecell[c]{RefineNet-\\Res101}  \\
\midrule
UM teacher & $rgb$ & 42.41 & 44.18  \\
UM student & $rgb$ & 41.23 & 42.89  \\
NOISY student & $rgb$ & 43.21 & 45.69 \\
MM student & $rgb, d$ & \textbf{45.71} & \textbf{46.95}  \\
\bottomrule
\end{tabular}
\caption{Ablation study for UM teacher model architecture. MM student consistently denoises pseudo labels when teacher model varies.} 
\label{tab:ablation-teacher}
\end{table}

\begin{table}[!htbp]
\centering
\begin{tabular}{cccc}
\toprule
Method & \textit{mod} & \makecell[c]{Labels for \\distilling} & Test mIoU(\%) \\
\midrule
UM teacher & $rgb$ & $\star$ & 44.18  \\
UM student & $rgb$ & hard  & 42.53  \\
UM student & $rgb$ & soft & 42.89  \\
MM student & $rgb, d$ & hard & 46.64   \\
MM student & $rgb, d$ & soft & \textbf{46.95}  \\
\bottomrule
\end{tabular}
\caption{Ablation study for hard \textit{vs.} soft labels on semantic segmentation. $\star$ means that the UM teacher is trained on true labels. Other methods are trained on pseudo labels generated by the UM teacher.} 
\label{tab:ablation-labels}
\end{table}

Despite different model architectures of the UM teacher, the conclusion holds same: MM student significantly outperforms the UM teacher and UM student, achieving knowledge expansion. In addition, a stronger teacher (\ie, more reliable pseudo labels) will lead to a better student model in the case of both unimodality and multimodality. Another observation here is that UM student fails to surpass UM teacher due to limited size of $D_u$. On the contrary, given small amount of unlabeled data, our MM student effectively utilizes unlabeled multimodal data and outperforms NOISY student which has access to both labeled and unlabeled data.

\subsection{Pseudo Labels for Distilling}

We also investigate how soft and hard pseudo labels influence results and report results in Table \ref{tab:ablation-labels}. We follow same data and model settings in the previous section.

As shown in Table \ref{tab:ablation-labels}, soft labels yield slightly better results than hard labels. The MM student learning from soft labels of the UM teacher achieves highest test mIoU.
