# Supplementary material for: Multimodal Knowledge Expansion
Source: arXiv:2103.14431 source file (2021-10-29)
Supplement: Supplementary file 3 [file supp4-proof.tex]

\section{Proofs}
\subsection{Equivalence of Loss Terms}
We prove below that Equation (\ref{eq:eqv}) is equivalent to Equation (3) in the main paper.
\begin{equation}
    \theta_s^\star = \argmin_{\theta_s} \frac1 M \sum_{i=1}^M l_{cls}(\tilde{\mathbf{y}}_i, \mathcal{T}(\mathbf{f}_s(\mathbf{x}_i^\alpha, \mathbf{x}_i^\beta;\theta_s))
\label{eq:eqv}
\end{equation}

$l_{cls}$ refers to cross entropy loss for hard labels and KL divergence loss for soft labels. It takes the form of:
\begin{equation}
    \begin{aligned}
        l_{cls}(y, p) = - \sum_{k=1}^{K} y_k \log \frac{\exp{p_k}}{\sum_{j=1}^{K} \exp{p_j}} + \sum_{k=1}^{K} y_k \log {y_k}
    \end{aligned}
\end{equation}
where $y$ and $p$ are $K$-dimensional vectors. $K$ denotes the number of classes. For simplicity, let  $z$ denote the output of feeding $p$ into a softmax layer, \ie, $\forall k\in [K], z_k = \frac{\exp{p_k}}{\sum_{j=1}^{K} \exp{p_j}}$. 
\vspace{1mm}

The derivative of $l_{cls}(y, p)$ with respect to $p_j$ is:
\begin{equation}
\begin{aligned}
    \frac{\partial{l_{cls}(y, p)}} {\partial{p_j}} &= -\sum_{k=1}^{K} y_k \frac{\partial{\log{z_k}}} {\partial{p_j}} \\
    & = -\sum_{k=1}^{K} y_k (I_{kj} - z_j) = z_j - y_j
\end{aligned}
\end{equation}

Therefore, $\triangledown {l_{cls}} = [z_1-y_1, z_2-y_2, ..., z_k-y_k]$.
\begin{equation}
    ||\triangledown {l_{cls}}|| = \sqrt{\sum_{j=1}^K (y_j-z_j)^2} \leq \sqrt{K}
    \label{eq:lip}
\end{equation}

Equation (\ref{eq:lip}) states that $l_{cls}(y, p)$ is Lipschitz continuous in $p$ for fixed $y$ with respect to $||\cdot||$, where $\sqrt{K}$ is the Lipschitz constant. Therefore, $\exists -\sqrt{K} \leq \gamma \leq \sqrt{K}$, such that loss terms in Equation (\ref{eq:eqv}) equal to that of Equation (3) in the main paper.

\subsection{Lemma 1}
To start with, by definition of ($a, c$) expansion and $max(c_1,c_2)\leq\frac{1}{\bar{a}}$, we derive Equation (\ref{eq:ac1}) and (\ref{eq:ac2}) from Equation (10) and (11) in the main paper.
\begin{equation}
    \label{eq:ac1}
    \begin{aligned}
	P_i(N(V^{\alpha})) & \geq c_1 P_i(V^{\alpha}) \\
&\forall \ V^{\alpha} \subseteq \mathcal X^{\alpha} \ with \ P_i(V^{\alpha}) \leq \bar{a}
\end{aligned}
\end{equation}

\begin{equation}
    \label{eq:ac2}
    \begin{aligned}
P_i(N(V^{\beta})) & \geq c_2 P_i(V^{\beta}) \\
&\forall \ V^{\beta} \subseteq \mathcal X^{\beta} \ with \ P_i(V^{\beta}) \leq \bar{a}
\end{aligned}
\end{equation}

Multiplying both sides of Equation (\ref{eq:ac1}) and Equation (\ref{eq:ac2}), we have:
\begin{equation}
    \label{eq:acmid}
    \begin{aligned}
	P_i(N(V^{\alpha}))& P_i(N(V^{\beta})) \geq c_1 c_2 P_i(V^{\alpha})P_i(V^{\beta}) \\
&\forall \ V^{\alpha} \subseteq \mathcal X^{\alpha} \ with \ P_i(V^{\alpha}) \leq \bar{a} \\
&\forall \ V^{\beta} \subseteq \mathcal X^{\beta} \ with \ P_i(V^{\beta}) \leq \bar{a}
\end{aligned}
\end{equation}

Plugging in conditional independence (\ie, Equation (12) in the main paper) gives us:  
\begin{equation}
    \label{eq:acfinal}
    \begin{aligned}
         P_i(N(V)) & \geq c_1 c_2 P_i(V), \\
         & \forall \ V \subseteq \mathcal X \ with \ P_i(V) \leq \bar{a}
    \end{aligned}
\end{equation}

Thus, $P$ on $\mathcal X$ satisfies ($\bar{a}, c_1c_2$) expansion.
