# Supplementary material for: Multimodal Knowledge Expansion
Source: arXiv:2103.14431 source file (2021-10-29)
Supplement: Supplementary file 4 [file supp1-data.tex]

\setcounter{section}{0}
\section{Dataset and Implementation Details}
% \subsection{TwoMoon Experiment}
% We generate 500 samples making two interleaving half circles. The dataset is randomly split as 30 labeled samples, 270 unlabeled samples and 200 test data (i.e., $|D_l|=30$, $|D_u|=270$, and $|D_{test}|=200$). Note that only one feature (i.e, X coordinates) of labeled data $D_l$ is accessible, while unlabeled data $D_u$ have both X and Y coordinates as features. 

\begin{figure*}[!htp]
\centering
\centering
\subfloat[UM teacher]{
\includegraphics[width=0.3\textwidth]{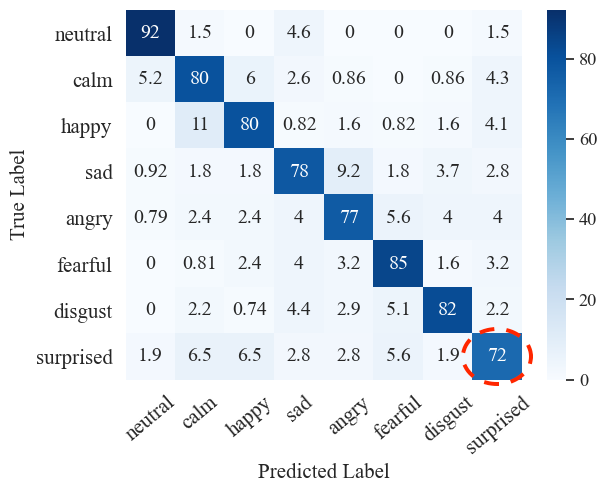}
\label{fig:emo-a}
%\caption{fig1}
}
\quad
\subfloat[NOISY student]{
\includegraphics[width=0.3\textwidth]{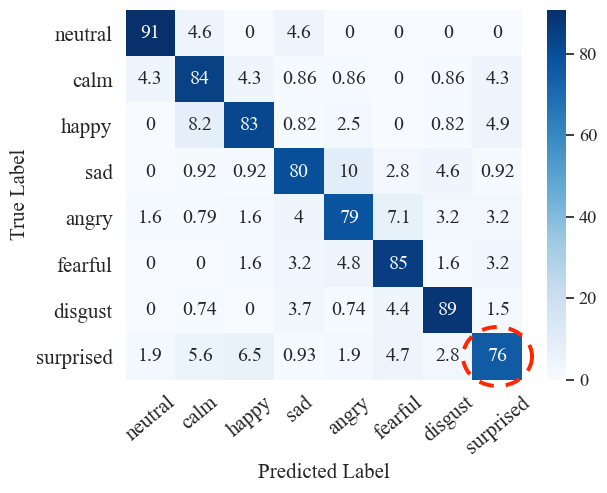}
\label{fig:emo-b}
}
\quad
\subfloat[MM student]{
\includegraphics[width=0.3\textwidth]{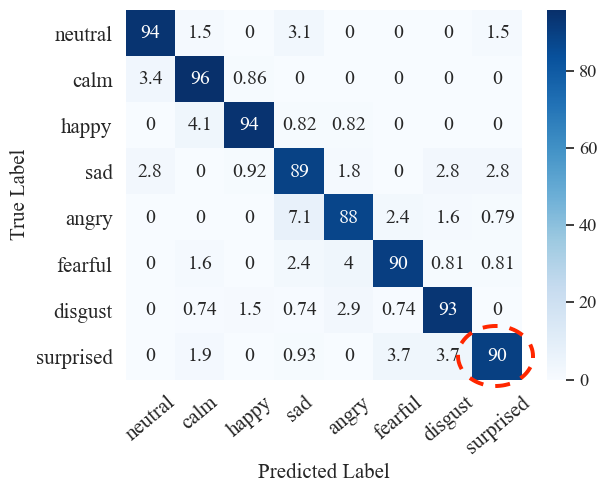}
\label{fig:emo-c}
}

\caption{normalized confusion matrix test accuracy}
\label{fig:emo}
\end{figure*}

\subsection{Emotion Recognition}
The Ryerson Audio-Visual Database of Emotional Speech and Song (RAVDESS) contains videos and audios of 24 professional actors (12 female, 12 male), vocalizing two lexically-matched statements. It contains 1440 emotional utterances with 8 different emotion classes: neutral, calm, happy, sad, angry, fearful, disgust and surprise. The dataset is randomly split as 2:8 for $D_l$ and $D_u$ and 8:1:1 as train / validation / test for $D_u$. To construct the labeled uni-modal dataset $D_l$, we select images every 0.5 second of a video clip as modality $\alpha$ and train a facial emotion recognition (FER) network as the UM teacher, which classifies emotions based on images. Image-audio pairs from video clips consist of the unlabeled multimodal dataset $D_u$. We sample images as inputs from modality $\alpha$ in the same way, adopt "Kaiser best" sampling for audios and take Mel-frequency cepstral coefficients (MFCCs) as inputs from modality $\beta$. 
% Hard pseudo labels given by the UM teacher are adopted.

\subsection{Semantic Segmentation}
NYU Depth V2 contains 1449 RGB-D images with 40-class labels, where 795 RGB images are adopted for training the UM teacher and the rest 654 RGB-D images are for testing. Besides labeled data, NYU Depth V2 also provides unannotated video sequences. We randomly sample 1488 RGB-D images as $D_u$ for training the student. Soft labels of the UM teacher are adopted. 

In addition, we propose a confidence-weighted loss term in this task to further regularize the student, preventing it from overfiting to the teacher. For each sample pixel $\mathbf{x}$ and its soft pseudo label $\tilde{\mathbf{y}}$, we assign $\mathbf{x}$ with a weight $\omega(\mathbf{x})$ defined by:
\begin{equation}
    \omega(\mathbf{x}) = 1 - \frac{\sum_{k=1}^K \tilde{\mathbf{y}}_i \log \tilde{\mathbf{y}}_i}{\log K}
\end{equation}
$K$ denotes the number of classes. We then modify $\mathcal{L}_{pl}$ in Equation (4) of the main paper by applying a weight for each sample:
\begin{equation}
    \mathcal{L}_{pl} = \frac1 M \sum_{i=1}^M \omega(\mathbf{x}) \  l_{cls}(\tilde{\mathbf{y}}_i,  \mathbf{f}_s(\mathbf{x}_i^\alpha, \mathbf{x}_i^\beta;\theta_s) \label{eq:l_pl})
\end{equation}

Figure \ref{fig:conf} demonstrates one image and its confidence map (\ie, $\omega(\mathbf x)$) based on pseudo labels of the UM teacher. Low confidence pixels are given a small weight while high confidence ones contribute largely in calculating the loss. This technique helps further reduce noise brought by inaccurate pseudo labels.

\begin{figure}[H]
\centering
\includegraphics[width=0.5\textwidth]{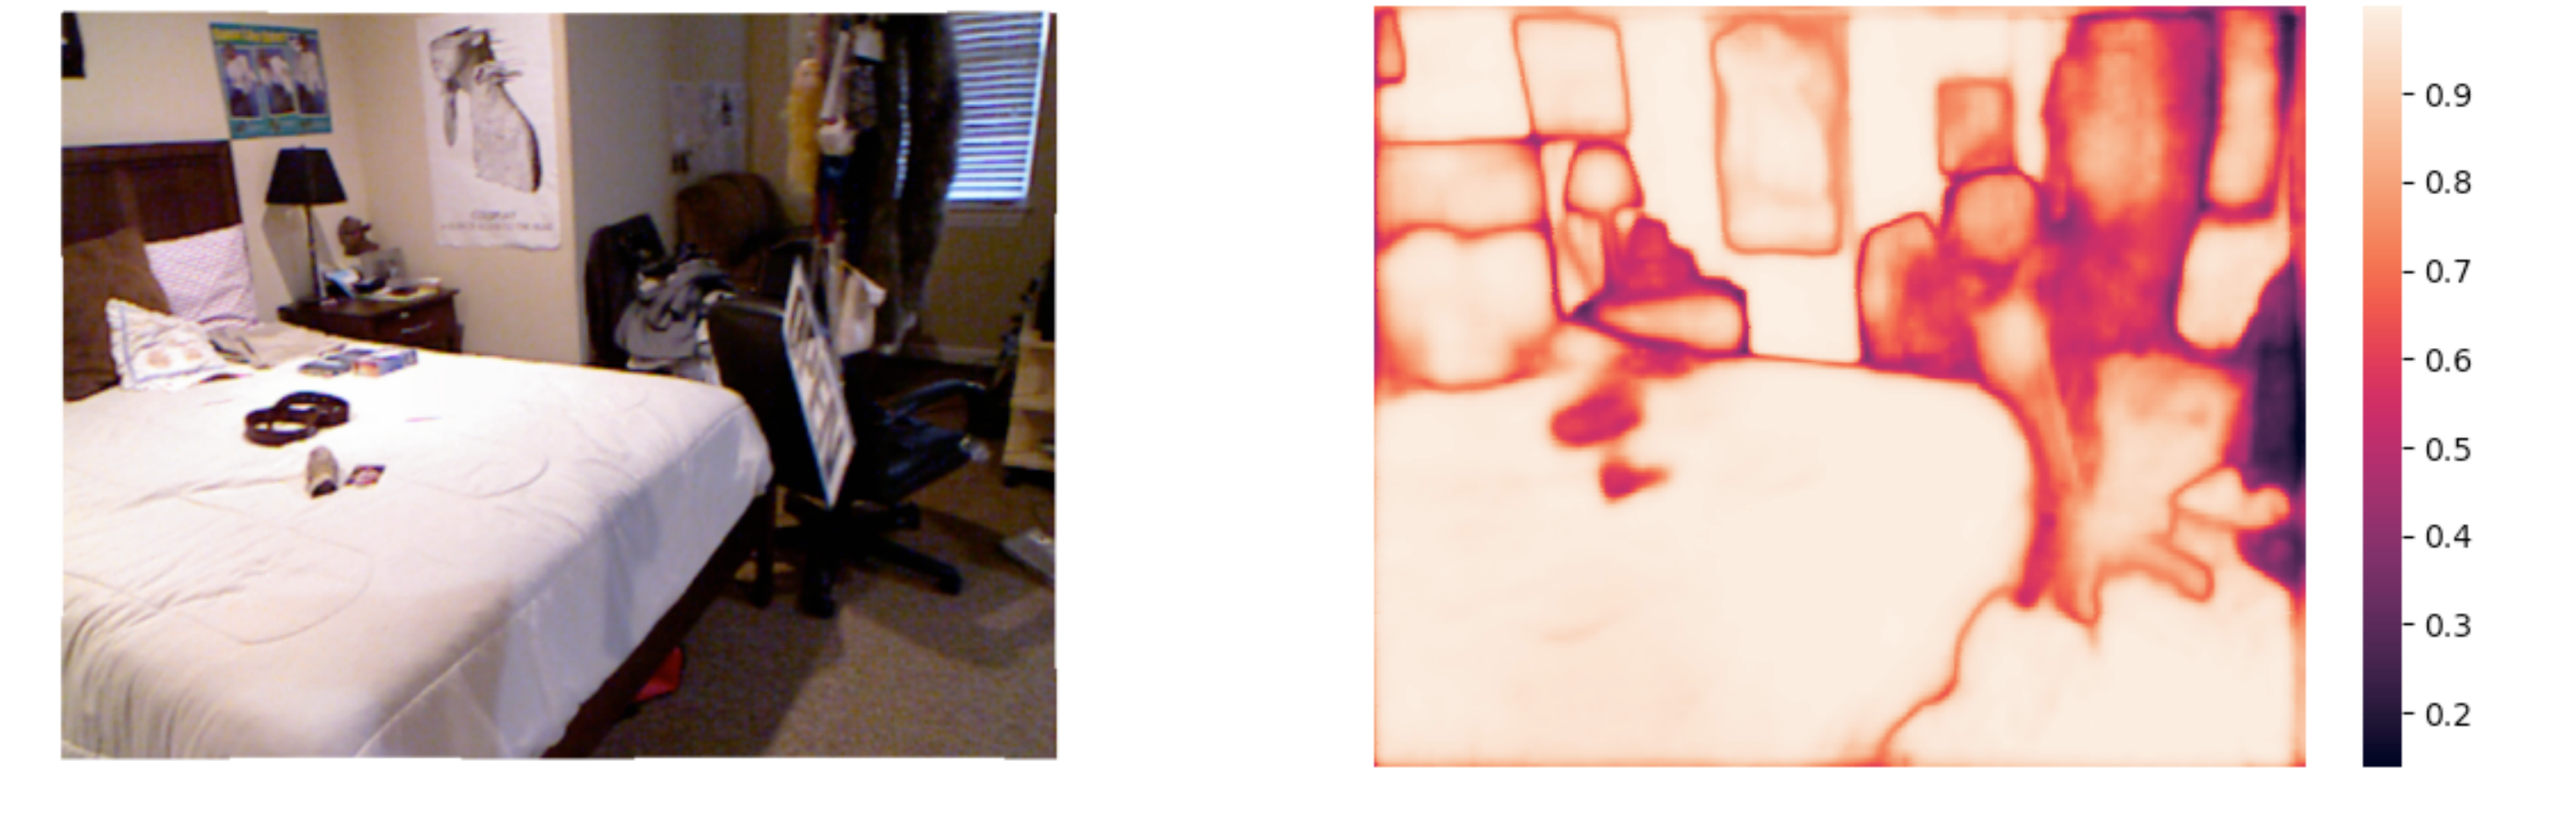} 
\caption{Left figure: one RGB image; right figure: corresponding weight value $\omega$ of each pixel.} 
\label{fig:conf} 
\end{figure}

\subsection{Event Classification}
The AudioSet and VGGSound are both audio-visual datasets for event classification. We take a mini common set of them including 3710 data in AudioSet and 3748 data for training and 1937 data for testing in VGGSound with 46 event categories. VGGSound guarantees the audio-video correspondence as the sound source is visually evident within the video, while AudioSet does not. Therefore, we consider AudioSet as a unimodal dataset and VGG Sound as multimodal. Audios from AudioSet and audio-video pairs from VGGSound are taken as the labeled unimodal dataset $D_l$ and unlabeled multimodal data $D_u$ respectively. Similarly, a student network is given soft pseudo labels of the UM teacher for training.
